# Supplementary material for: funBIalign: a hierachical algorithm for functional motif discovery based on mean squared residue scores
Source: arXiv:2306.04254 ancillary file (2023-06-07)
Supplement: Supplementary file 1 [file funBIalign_supplement.pdf]

# ***funBAlign*: a hierarchical algorithm for functional motif discovery based on mean squared residue score - Supplementary Material**

Jacopo Di Iorio  
Dept. of Statistics, Penn State University

Marzia A. Cremona  
Dept. of Operations and Decision Systems, Université Laval

Francesca Chiaromonte  
Dept. of Statistics, Penn State University

June 5, 2023

## **S1 Proof of Theorem 1**

*Proof.* Given a functional motif  $Q$  composed of  $n_Q$  portions, the functional mean squared residue score is defined as

$$H(Q) = \frac{1}{n_Q} \frac{1}{l} \sum_{k=1}^{n_Q} \int_0^l (p_k(t) - \bar{p}_k - \bar{p}(t) + \bar{p})^2 dt,$$

where we have

$$\begin{aligned}\bar{p}_k &= \frac{1}{l} \int_0^l p_k(t) dt, \\ \bar{p}(t) &= \frac{1}{n_Q} \sum_{k=1}^{n_Q} p_k(t), \\ \bar{p} &= \frac{1}{n_Q} \frac{1}{l} \sum_{k=1}^{n_Q} \int_0^l p_k(t) dt.\end{aligned}$$

We define  $g_k(t) := p_k(t) - \bar{p}_k - \bar{p}(t) + \bar{p}$ , so that  $H(Q) = \frac{1}{n_Q} \frac{1}{l} \sum_{k=1}^{n_Q} \int_0^l g_k^2(t) dt$ . We have that:

$$\begin{aligned} g_k(t) &= p_k(t) - \bar{p}_k - \frac{1}{n_Q} \sum_{j=1}^{n_Q} p_j(t) + \frac{1}{n_Q} \sum_{j=1}^{n_Q} \bar{p}_j \\ &= \frac{n_Q - 1}{n_Q} p_k(t) - \frac{n_Q - 1}{n_Q} \bar{p}_k - \frac{1}{n_Q} \sum_{j \neq k} p_j(t) + \frac{1}{n_Q} \sum_{j \neq k} \bar{p}_j \\ &= A + B + C + D. \end{aligned}$$

Then  $g_k^2(t)$  is:

$$g_k^2(t) = A^2 + B^2 + C^2 + D^2 + 2AB + 2AC + 2AD + 2BC + 2BD + 2CD$$

where

$$\begin{aligned} A^2 &= \frac{(n_Q - 1)^2}{n_Q^2} p_k^2(t), \\ B^2 &= \frac{(n_Q - 1)^2}{n_Q^2} \bar{p}_k^2, \\ C^2 &= \frac{1}{n_Q^2} \sum_{j \neq k} p_j^2(t) + \frac{1}{n_Q^2} \sum_{j \neq k} \left( p_j(t) \sum_{i \neq \{j, k\}} p_i(t) \right), \\ D^2 &= \frac{1}{n_Q^2} \sum_{j \neq k} \bar{p}_j^2 + \frac{1}{n_Q^2} \sum_{j \neq k} \left( \bar{p}_j \sum_{i \neq \{j, k\}} \bar{p}_i \right), \\ 2AB &= -2 \frac{(n_Q - 1)^2}{n_Q^2} p_k(t) \bar{p}_k, \\ 2AC &= -2 \frac{n_Q - 1}{n_Q^2} p_k(t) \sum_{j \neq k} p_j(t), \\ 2AD &= 2 \frac{n_Q - 1}{n_Q^2} p_k(t) \sum_{j \neq k} \bar{p}_j, \\ 2BC &= 2 \frac{n_Q - 1}{n_Q^2} \bar{p}_k \sum_{j \neq k} p_j(t), \\ 2BD &= -2 \frac{n_Q - 1}{n_Q^2} \bar{p}_k \sum_{j \neq k} \bar{p}_j, \\ 2CD &= -2 \frac{1}{n_Q^2} \left( \sum_{j \neq k} p_j(t) \bar{p}_j \right). \end{aligned}$$

Defining  $z_k(t) := p_k^2(t)$ , we can rewrite  $A^2$  and  $C^2$  in the following way:

$$A^2 = \frac{(n_Q - 1)^2}{n_Q^2} z_k(t),$$

$$C^2 = \frac{1}{n_Q^2} \sum_{j \neq k} z_j(t) + \frac{1}{n_Q^2} \sum_{j \neq k} \left( p_j(t) \sum_{i \neq \{j, k\}} p_i(t) \right).$$

Noting that  $2\frac{1}{l} \int_0^l BC dt + 2\frac{1}{l} \int_0^l BD dt = 0$ , we can then compute:

$$\begin{aligned} \frac{1}{l} \int_0^l g_k^2(t) dt &= \frac{1}{l} \int_0^l A^2 dt + \frac{1}{l} \int_0^l B^2 dt \\ &\quad + \frac{1}{l} \int_0^l C^2 dt + \frac{1}{l} \int_0^l D^2 dt + \\ &\quad + 2\frac{1}{l} \int_0^l AB dt + 2\frac{1}{l} \int_0^l AC dt + 2\frac{1}{l} \int_0^l AD dt + 2\frac{1}{l} \int_0^l CD dt \\ &= \frac{(n_Q - 1)^2}{n_Q^2} \bar{z}_k + \frac{(n_Q - 1)^2}{n_Q^2} \bar{p}_k^2 \\ &\quad + \frac{1}{n_Q^2} \sum_{j \neq k} \bar{z}_j + \frac{1}{n_Q^2} \frac{1}{l} \int_0^l \sum_{j \neq k} \left( p_j(t) \sum_{i \neq \{j, k\}} p_i(t) \right) dt + \frac{1}{n_Q^2} \sum_{j \neq k} \bar{p}_j^2 + \frac{1}{n_Q^2} \sum_{j \neq k} \left( \bar{p}_j \sum_{i \neq \{j, k\}} \bar{p}_i \right) + \\ &\quad - 2\frac{(n_Q - 1)^2}{n_Q^2} \bar{p}_k^2 - 2\frac{n_Q - 1}{n_Q^2} \frac{1}{l} \int_0^l \left( p_k(t) \sum_{j \neq k} p_j(t) \right) dt + 2\frac{n_Q - 1}{n_Q^2} \bar{p}_k \sum_{j \neq k} \bar{p}_j - 2\frac{1}{n_Q^2} \left( \sum_{j \neq k} \bar{p}_j \right)^2. \end{aligned}$$

We now compute the coefficients corresponding to each of the elements  $\bar{z}_\kappa$ ,  $\bar{p}_\kappa^2$ ,  $\frac{1}{l} \int_0^l p_\kappa(t) p_\iota(t) dt$ , and  $\bar{p}_\kappa \bar{p}_\iota$ , with  $\iota \neq \kappa$ , in the H-score of a motif  $Q$  composed of  $n_Q$  portions, multiplied by  $n_Q$ :

$$\begin{aligned} n_Q H(Q) &= \sum_{k=1}^{n_Q} \frac{1}{l} \int_0^l g_k^2(t) dt \\ &= \sum_{\kappa=1}^{n_Q} \left[ h_{\bar{z}_\kappa}^Q \bar{z}_\kappa + h_{\bar{p}_\kappa^2}^Q \bar{p}_\kappa^2 + \sum_{\iota \neq \kappa} \left( h_{\frac{1}{l} \int_0^l p_\kappa(t) p_\iota(t) dt}^Q \frac{1}{l} \int_0^l p_\kappa(t) p_\iota(t) dt + h_{\bar{p}_\kappa \bar{p}_\iota}^Q \bar{p}_\kappa \bar{p}_\iota \right) \right]. \end{aligned}$$

We start computing  $h_{\bar{z}_\kappa}^Q$ , the coefficient referring to  $\bar{z}_\kappa$ . This element appears twice: in  $\frac{(n_Q - 1)^2}{n_Q^2} \bar{z}_k$  when  $k = \kappa$ , and in  $\frac{1}{n_Q^2} \sum_{j \neq k} \bar{z}_j$  when  $k \neq \kappa$  (that is,  $n_Q - 1$  times). Hence, we have

$$h_{\bar{z}_\kappa}^Q = \frac{(n_Q - 1)^2}{n_Q^2} + \frac{n_Q - 1}{n_Q^2} = \frac{n_Q - 1}{n_Q}.$$

To compute the coefficient  $h_{\bar{p}_\kappa^2}^Q$  referring to the element  $\bar{p}_\kappa^2$ , we need to consider that the element appears four times: in  $\frac{(n_Q - 1)^2}{n_Q^2} \bar{p}_k^2$  and in  $-2\frac{(n_Q - 1)^2}{n_Q^2} \bar{p}_k^2$  when  $k = \kappa$ ; in  $\frac{1}{n_Q^2} \sum_{j \neq k} \bar{p}_j^2$  and in

$-2\frac{1}{n_Q^2} \left( \sum_{j \neq k} \bar{p}_j \right)^2$  when  $k \neq \kappa$  (that is,  $n_Q - 1$  times). Hence, we have

$$h_{\bar{p}_\kappa}^Q = \frac{(n_Q - 1)^2}{n_Q^2} - 2\frac{(n_Q - 1)^2}{n_Q^2} + \frac{n_Q - 1}{n_Q^2} - 2\frac{n_Q - 1}{n_Q^2} = -\frac{n_Q - 1}{n_Q}.$$

For the coefficient of the element  $\frac{1}{l} \int_0^l p_\kappa(t) p_\iota(t) dt$  for  $\iota \neq \kappa$ , i.e.  $h_{\bar{p}_{\iota\kappa}}^Q$ , we need to consider the term  $-2\frac{n_Q-1}{n_Q^2} \frac{1}{l} \int_0^l \left( p_\kappa(t) \sum_{j \neq k} p_j(t) \right) dt$  when  $k = \kappa$  or  $k = \iota$  (that is, 2 times), and the term  $\frac{1}{n_Q^2} \frac{1}{l} \int_0^l \sum_{j \neq k} \left( p_j(t) \sum_{i \neq \{j, k\}} p_i(t) \right) dt$  when  $k \neq \{\kappa, \iota\}$  (that is,  $2(n_Q - 2)$  times). We obtain:

$$h_{\bar{p}_{\iota\kappa}}^Q = -2 \left( -2\frac{n_Q - 1}{n_Q^2} \right) + 2\frac{n_Q - 2}{n_Q^2} = -\frac{2}{n_Q}.$$

Finally, we compute  $h_{\bar{p}_\kappa \bar{p}_\iota}^Q$  for  $\iota \neq \kappa$ , the coefficient corresponding to  $\bar{p}_\kappa \bar{p}_\iota$ . This element appears in the term  $2\frac{n_Q-1}{n_Q^2} \bar{p}_k \sum_{j \neq k} \bar{p}_j$  when  $k \neq \kappa$  or  $k \neq \iota$  (that is, 2 times), in the term  $\frac{1}{n_Q^2} \sum_{j \neq k} \left( \bar{p}_j \sum_{i \neq \{j, k\}} \bar{p}_i \right)$  when  $k \neq \{\kappa, \iota\}$  (that is,  $2(n_Q - 2)$  times), and in the term  $-2\frac{1}{n_Q^2} \left( \sum_{j \neq k} \bar{p}_j \right)^2$  when  $k \neq \{\kappa, \iota\}$  (that is,  $2(n_Q - 2)$  times). Hence, we have:

$$h_{\bar{p}_\kappa \bar{p}_\iota}^Q = 2 \left( 2\frac{n_Q - 1}{n_Q^2} \right) + 2\frac{n_Q - 2}{n_Q^2} + 2(n_Q - 2) \left( -2\frac{1}{n_Q^2} \right) = \frac{2}{n_Q}.$$

We now consider  $\bar{H}_n$  for  $n = 2, 3, \dots, n_Q$ , the average fMRS of all  $\binom{n_Q}{n}$  sub-motifs of  $Q$  obtained selecting exactly  $n$  of the  $n_Q$  portions  $p_k(t)$  belonging to  $Q$ :

$$\begin{aligned} \bar{H}_n &= \binom{n_Q}{n}^{-1} \sum_{\substack{R \subseteq Q \\ |R|=n}} H(R) \\ &= \sum_{\kappa=1}^{n_Q} \left[ \bar{h}_{\bar{z}_\kappa}^n \bar{z}_\kappa + \bar{h}_{\bar{p}_\kappa^2}^n \bar{p}_\kappa^2 + \sum_{\iota \neq \kappa} \left( \bar{h}_{\bar{p}_{\iota\kappa}}^n \frac{1}{l} \int_0^l p_\kappa(t) p_\iota(t) dt + \bar{h}_{\bar{p}_\kappa \bar{p}_\iota}^n \bar{p}_\kappa \bar{p}_\iota \right) \right]. \end{aligned}$$

We start computing  $\bar{h}_{\bar{z}_\kappa}^n$ , the coefficient corresponding to  $\bar{z}_\kappa$ . This element appears in the  $H(R)$  of the sub-motifs comprising the portion  $p_\kappa(t)$ , that are exactly  $\binom{n_Q-1}{n-1}$ . Hence, we have:

$$\bar{h}_{\bar{z}_\kappa}^n = \frac{\binom{n_Q-1}{n-1}}{\binom{n_Q}{n}} \frac{h_{\bar{z}_\kappa}^R}{n} = \frac{n-1}{nn_Q}.$$

To compute  $\bar{h}_{\bar{p}_\kappa^2}^n$ , the coefficient of the element  $\bar{p}_\kappa^2$ , we need to consider the sub-motifs comprising the portion  $p_\kappa(t)$ . There are exactly  $\binom{n_Q-1}{n-1}$  such motifs, so we obtain:

$$\bar{h}_{\bar{p}_\kappa^2}^n = \frac{\binom{n_Q-1}{n-1}}{\binom{n_Q}{n}} \frac{h_{\bar{p}_\kappa^2}^R}{n} = -\frac{n-1}{nn_Q}.$$

To compute the coefficient  $\bar{h}_{\bar{p}_\iota\bar{p}_\kappa}^n$  of the element  $\frac{1}{l} \int_0^l p_\kappa(t)p_\iota(t)dt$  with  $\iota \neq \kappa$  we need to consider the  $\binom{n_Q-2}{n-2}$  sub-motifs comprising both portions  $p_\kappa(t)$  and  $p_\iota(t)$ , obtaining:

$$\bar{h}_{\bar{p}_\iota\bar{p}_\kappa}^n = \frac{\binom{n_Q-2}{n-2}}{\binom{n_Q}{n}} \frac{h_{\bar{p}_\iota\bar{p}_\kappa}^R}{n} = -2 \frac{n-1}{n_Q(n_Q-1)n}.$$

Finally, for the coefficient  $\bar{h}_{\bar{p}_\kappa\bar{p}_\iota}^n$  corresponding to the element  $\bar{p}_\kappa\bar{p}_\iota$  with  $\iota \neq \kappa$ , we need to consider the  $\binom{n_Q-2}{n-2}$  sub-motifs comprising both portions  $p_\kappa(t)$  and  $p_\iota(t)$ . Hence, we have:

$$\bar{h}_{\bar{p}_\kappa\bar{p}_\iota}^n = \frac{\binom{n_Q-2}{n-2}}{\binom{n_Q}{n}} \frac{h_{\bar{p}_\kappa\bar{p}_\iota}^R}{n} = 2 \frac{n-1}{n_Q(n_Q-1)n}.$$

Putting all the terms together, we obtain:

$$\bar{H}_n = \frac{n-1}{nn_Q} \sum_{\kappa=1}^{n_Q} \left[ \bar{z}_\kappa + \bar{p}_\kappa^2 - \frac{2}{n_Q-1} \sum_{\iota \neq \kappa} \left( \frac{1}{l} \int_0^l p_\kappa(t)p_\iota(t)dt - \bar{p}_\kappa\bar{p}_\iota \right) \right].$$

We are interested in the relationship between  $\bar{H}_{n+1}$  and  $\bar{H}_n$ . We have:

$$\begin{aligned} \bar{H}_{n+1} &= \frac{n}{(n+1)n_Q} \sum_{\kappa=1}^{n_Q} \left[ \bar{z}_\kappa + \bar{p}_\kappa^2 - \frac{2}{n_Q-1} \sum_{\iota \neq \kappa} \left( \frac{1}{l} \int_0^l p_\kappa(t)p_\iota(t)dt - \bar{p}_\kappa\bar{p}_\iota \right) \right] \\ &= \frac{n^2}{(n+1)(n-1)} \bar{H}_n, \end{aligned}$$

from which we obtain

$$\bar{H}_{n+1} = \bar{H}_n \frac{n^2}{n^2-1}.$$

□

## S2 A schematic of *funBAlign* algorithm

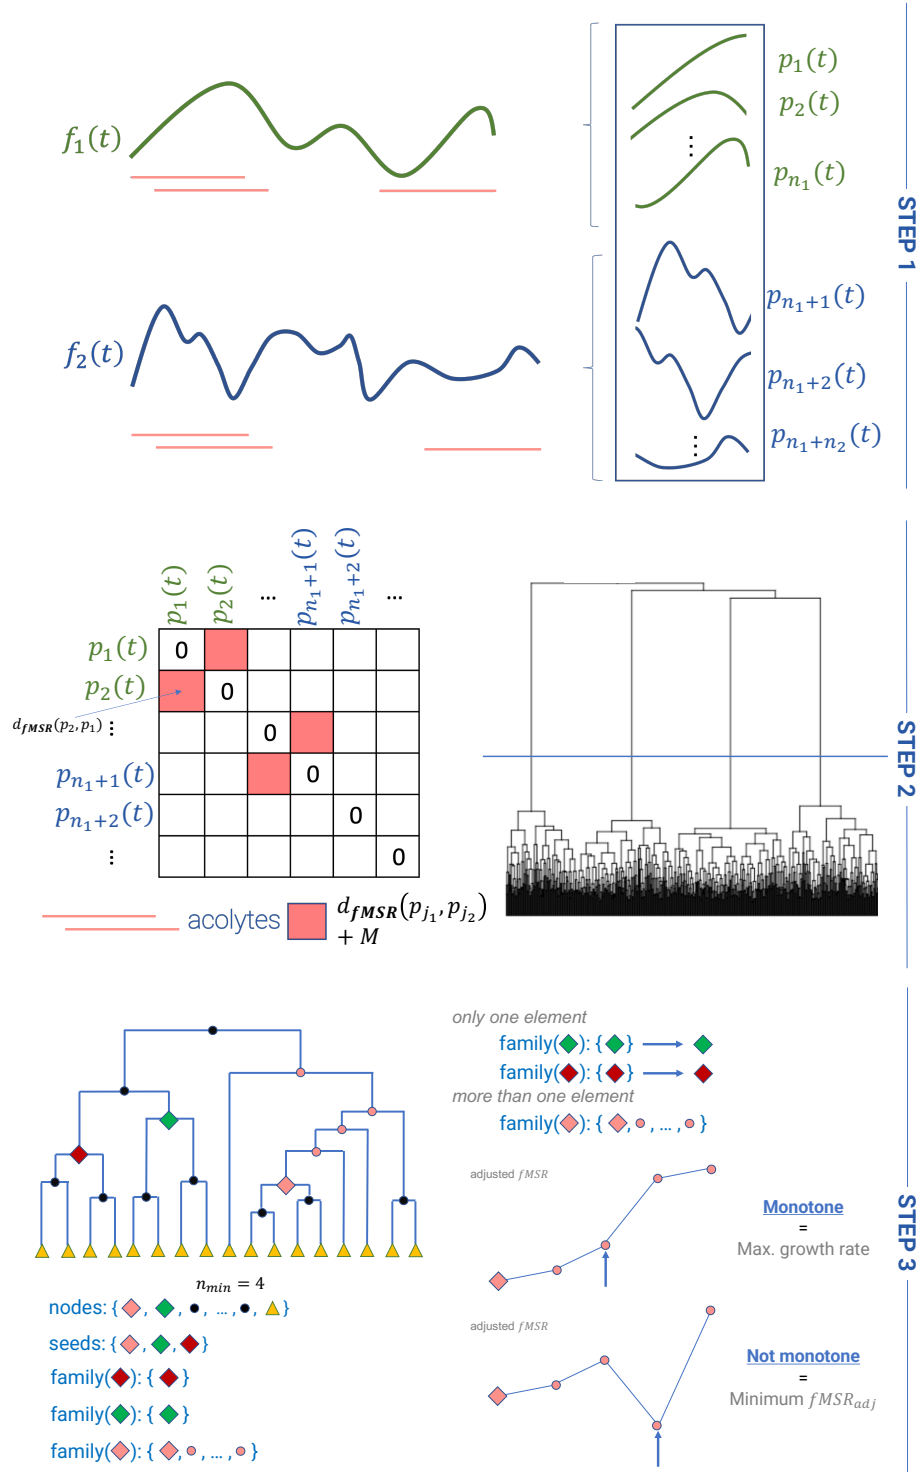

Figure S1: A visual scheme of the three main steps of *funBAlign* algorithm.

## S3 Motifs with shared noise level

### S3.1 Motifs with 8 occurrences

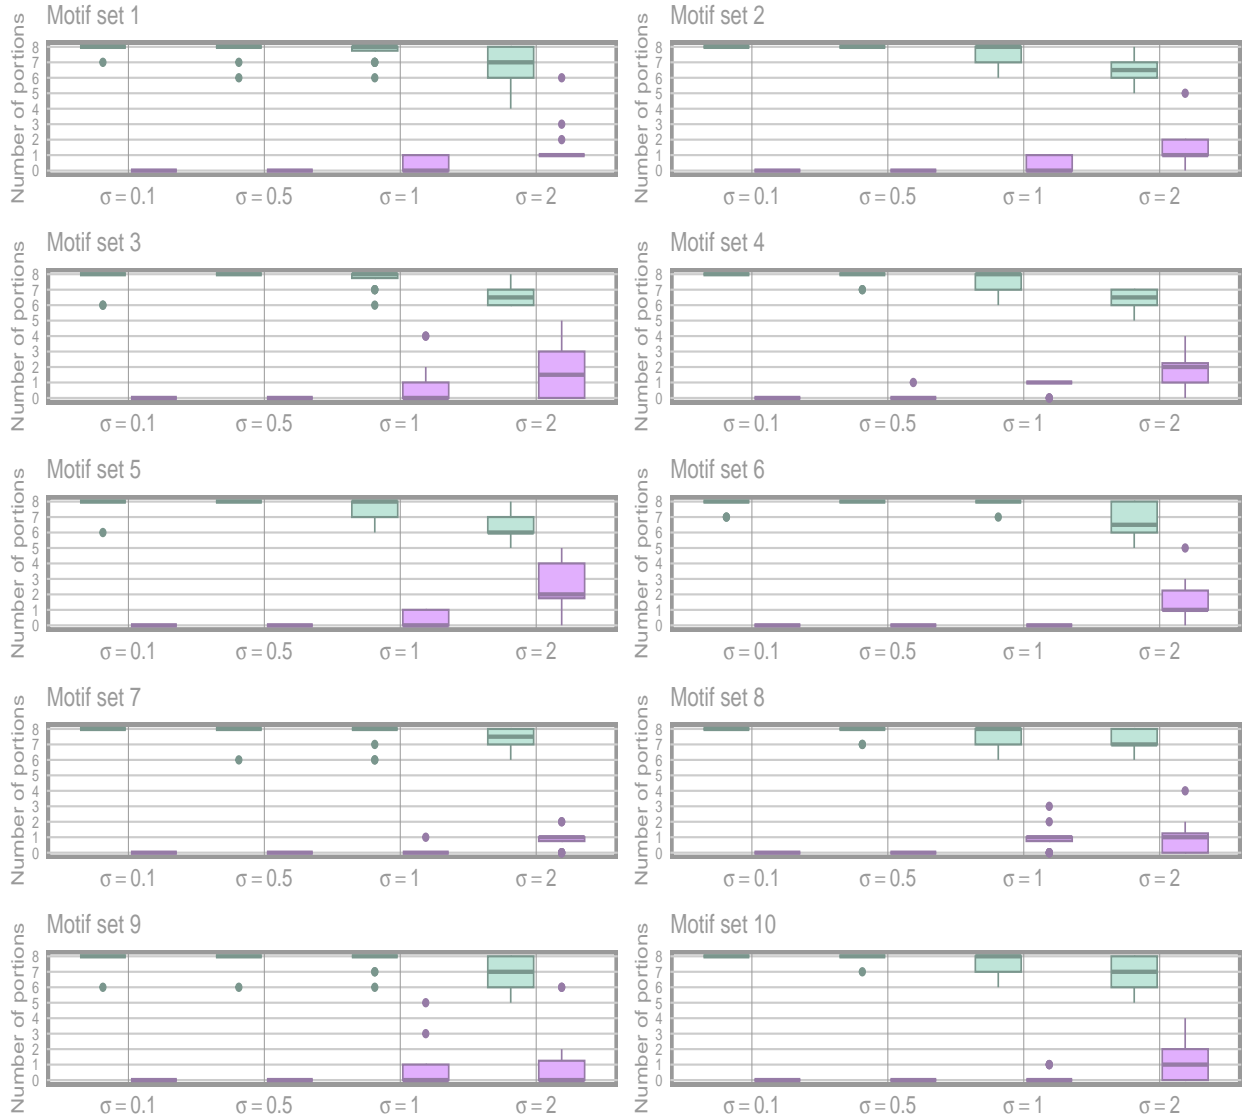

Figure S2: Performance of *funBIalign* for all simulations where motifs have 8 occurrences and shared noise level. Different panels show the performance pooling across runs of the algorithm with minimum cardinalities  $n_{min} = 5, 6, 7, 8$ , but separately for each of the 10 alternative motif sets. For each  $\sigma$ , the green and pink boxplots (left and right) represent correctly identified portions and extra portions, respectively.

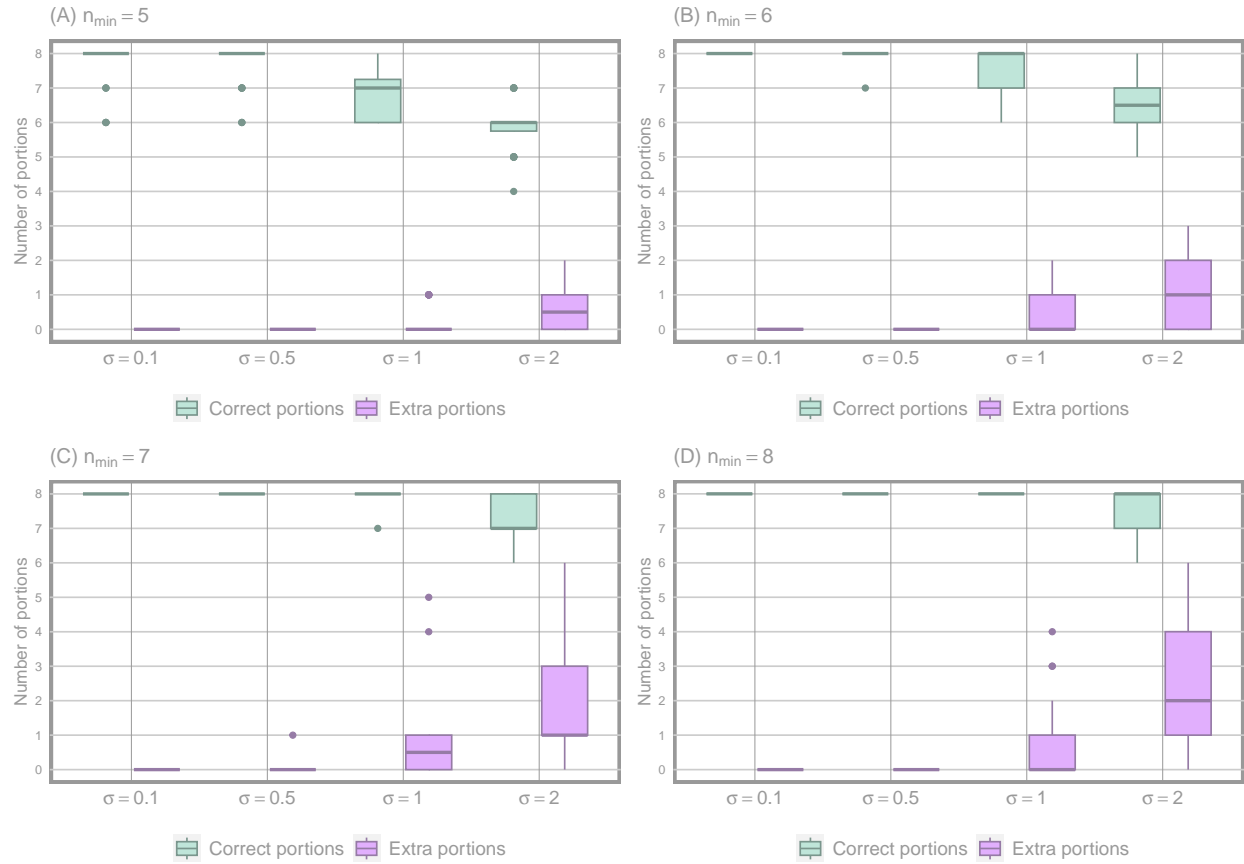

Figure S3: Performance of *funBIalign* for all simulations where motifs have 8 occurrences and shared noise level. The four panels show the performance of the algorithm run with minimum cardinalities  $n_{\min} = 5, 6, 7, 8$ , respectively, but pooling across 10 alternative motif sets. For each  $\sigma$ , the green and pink boxplots (left and right) represent correctly identified portions and extra portions, respectively.

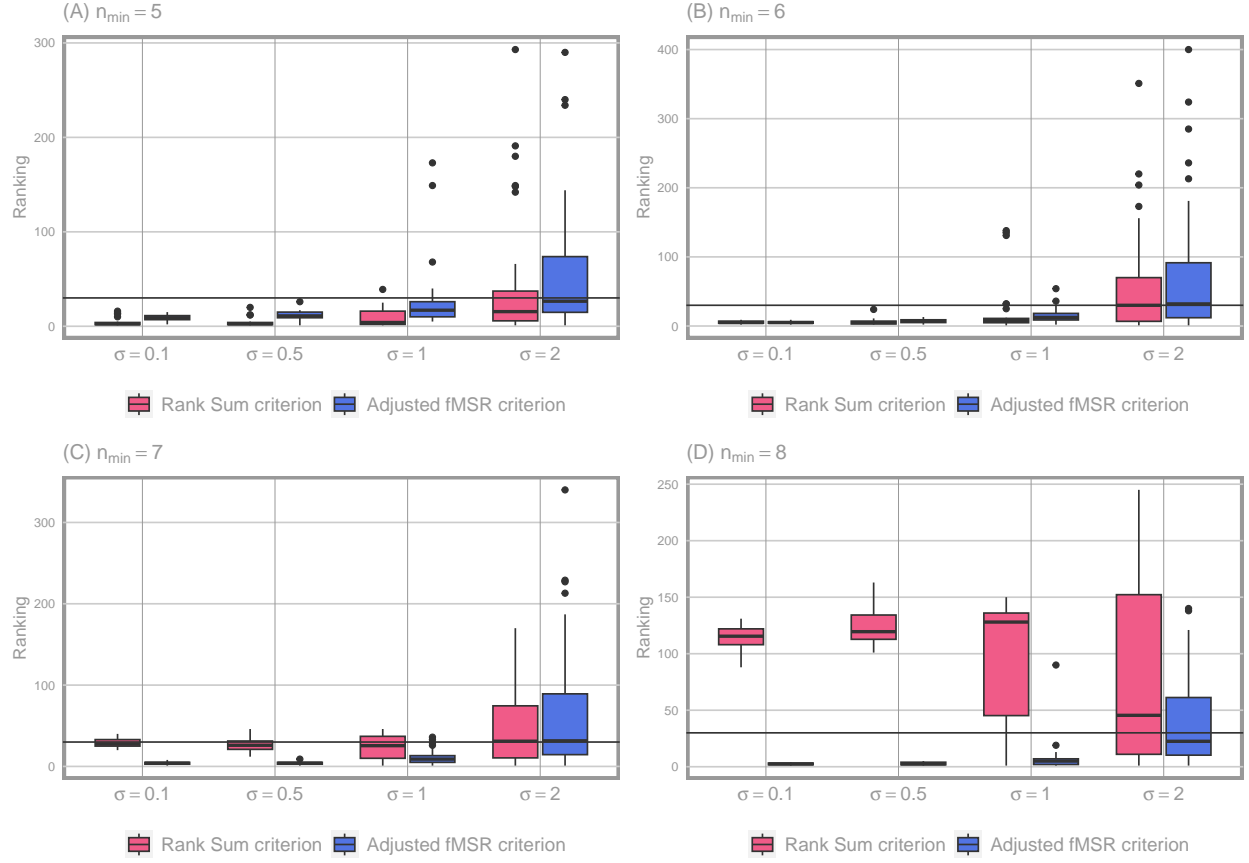

Figure S4: Ranking of the results of *funBAlign* which are most similar to the intentionally embedded motifs, for all simulations where motifs have 8 occurrences and shared noise level. The four panels show the ranking of the algorithm run with minimum cardinalities  $n_{\min} = 5, 6, 7, 8$ , respectively, but pooling across 10 alternative motif sets. For each  $\sigma$ , the red and blue boxplots (left and right) represent ranking according to the rank sum and the adjusted fMSR criterion, respectively. Horizontal line indicates rank 30.

### S3.2 Motifs with 10 occurrences

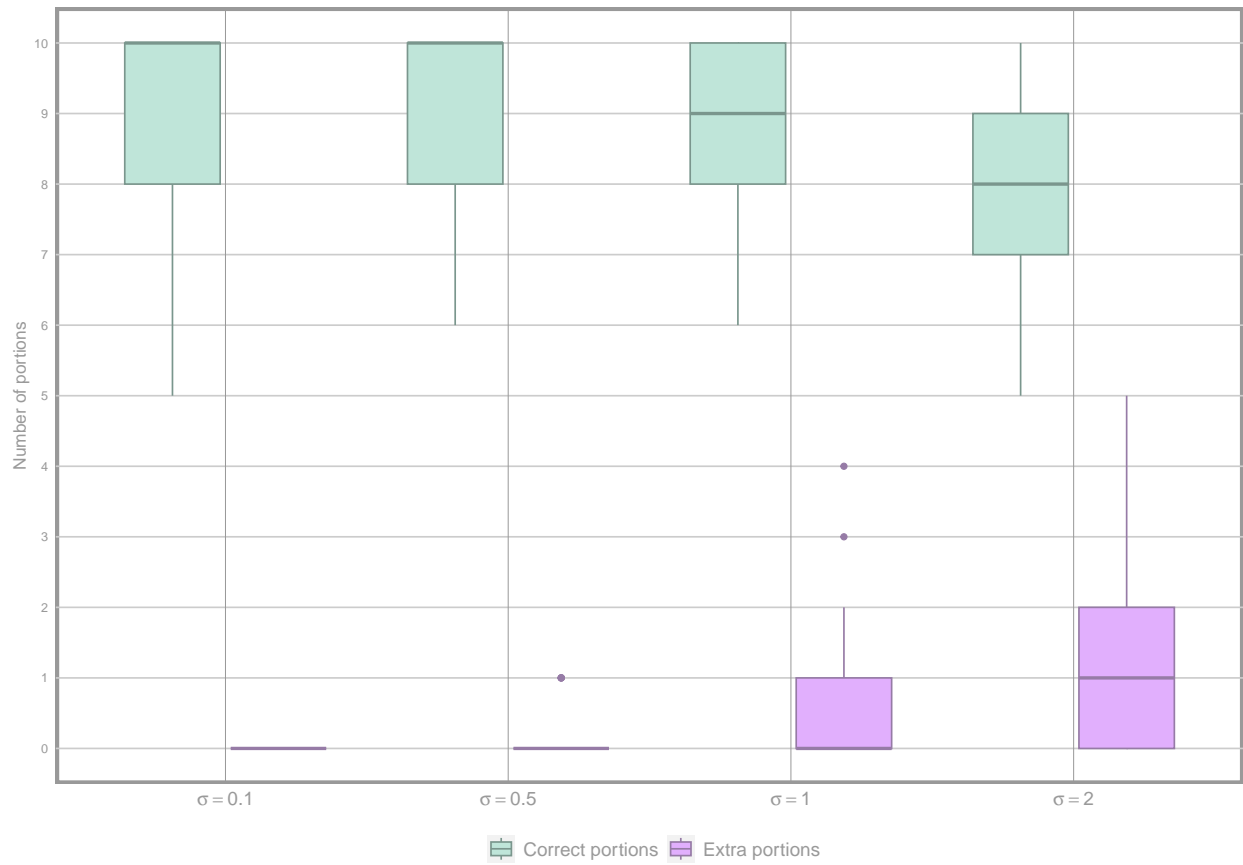

Figure S5: Performance of *funBAlign* for all simulations where motifs have 10 occurrences and shared noise levels. The algorithm is run with minimum cardinalities  $n_{min} = 5, 6, 7, 8$  and results are pooled. For each  $\sigma$ , the green and pink boxplots (left and right) represent correctly identified portions and extra portions, respectively. See Figure 2.A.

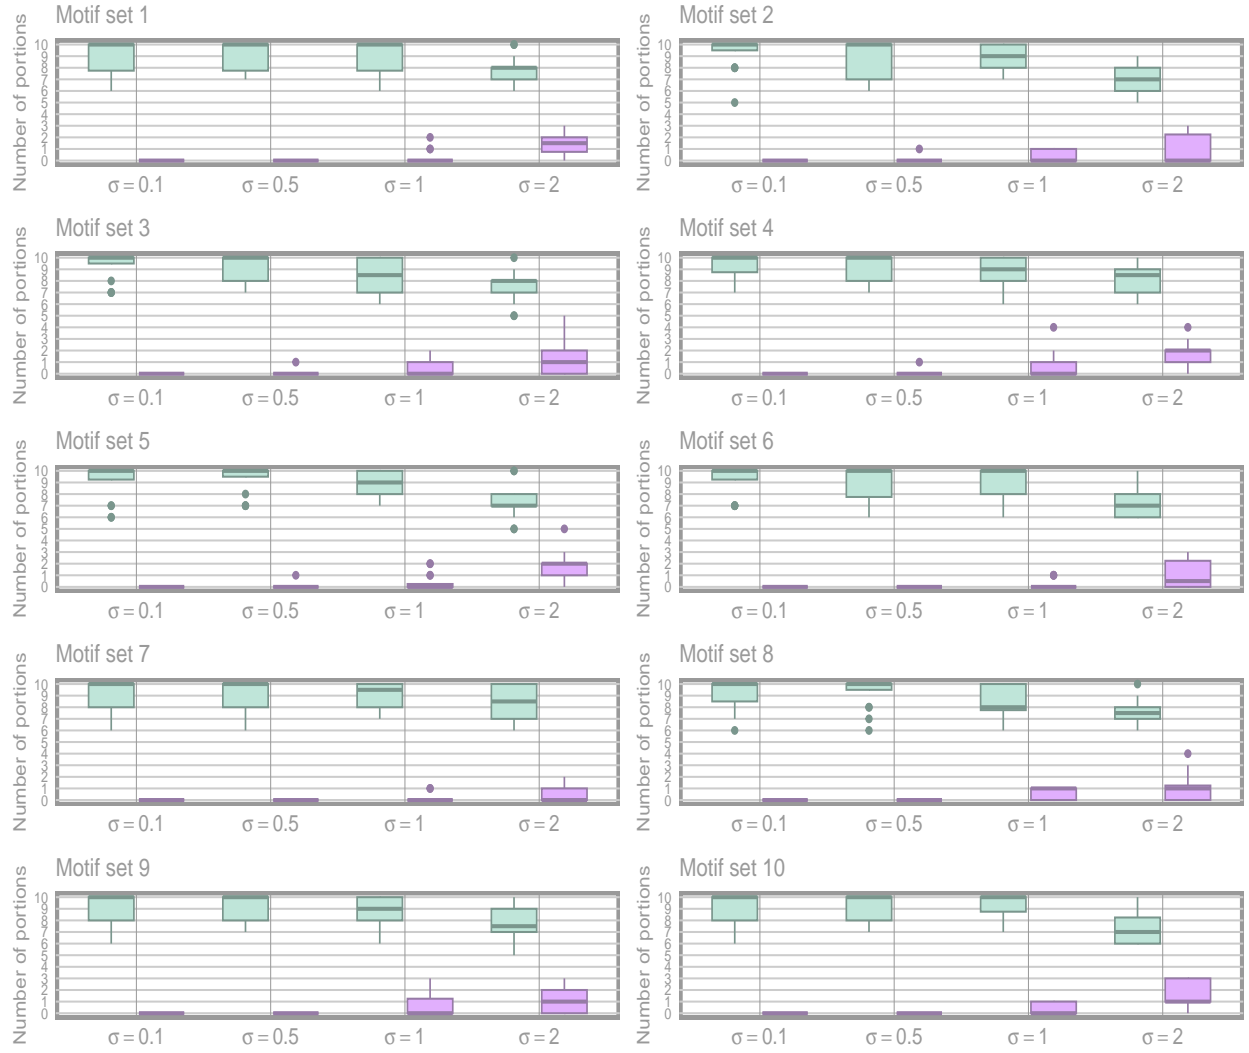

Figure S6: Performance of *funBAlign* for all simulations where motifs have 10 occurrences and shared noise level. Different panels show the performance pooling across runs of the algorithm with minimum cardinalities  $n_{min} = 5, 6, 7, 8$ , but separately for each of the 10 alternative motif sets. For each  $\sigma$ , the green and pink boxplots (left and right) represent correctly identified portions and extra portions, respectively.

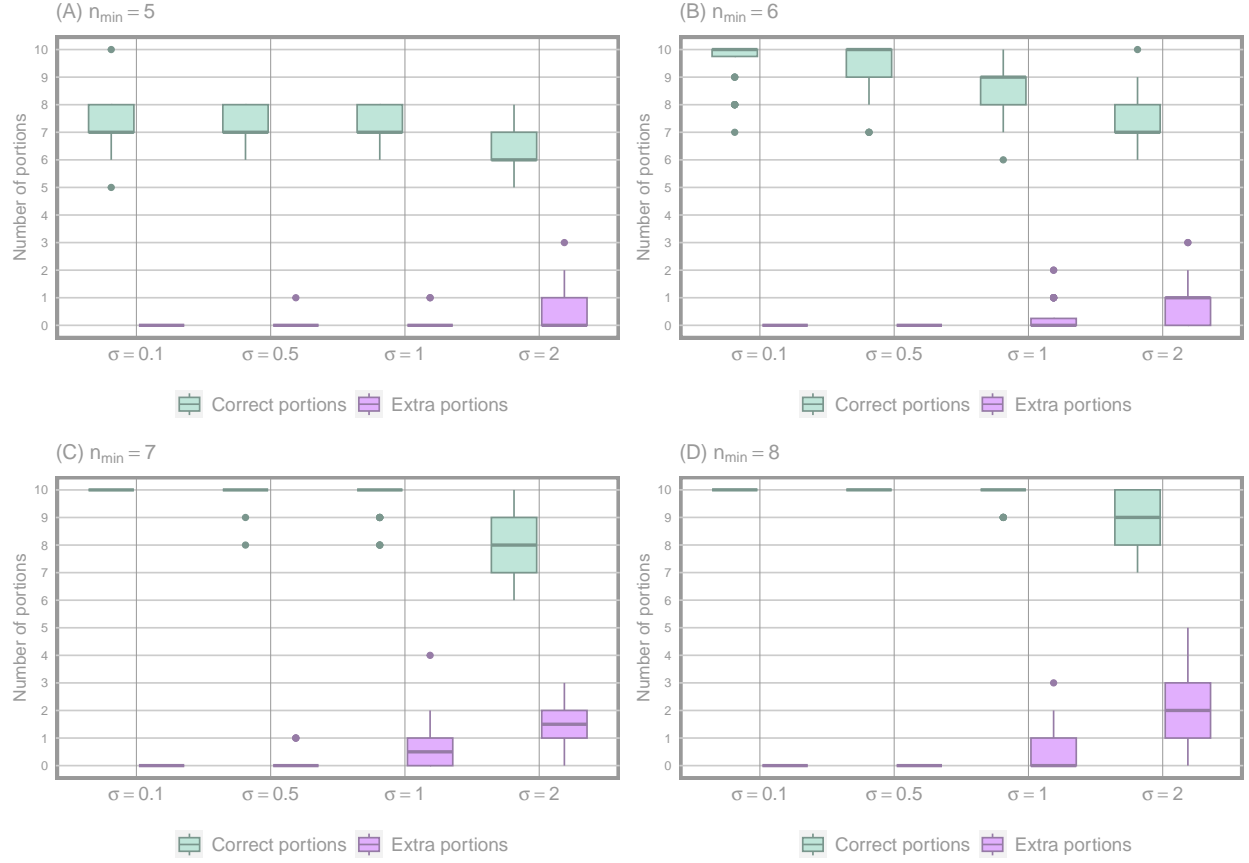

Figure S7: Performance of *funBIalign* for all simulations where motifs have 10 occurrences and shared noise level. The four panels show the performance of the algorithm run with minimum cardinalities  $n_{\min} = 5, 6, 7, 8$ , respectively, but pooling across 10 alternative motif sets. For each  $\sigma$ , the green and pink boxplots (left and right) represent correctly identified portions and extra portions, respectively.

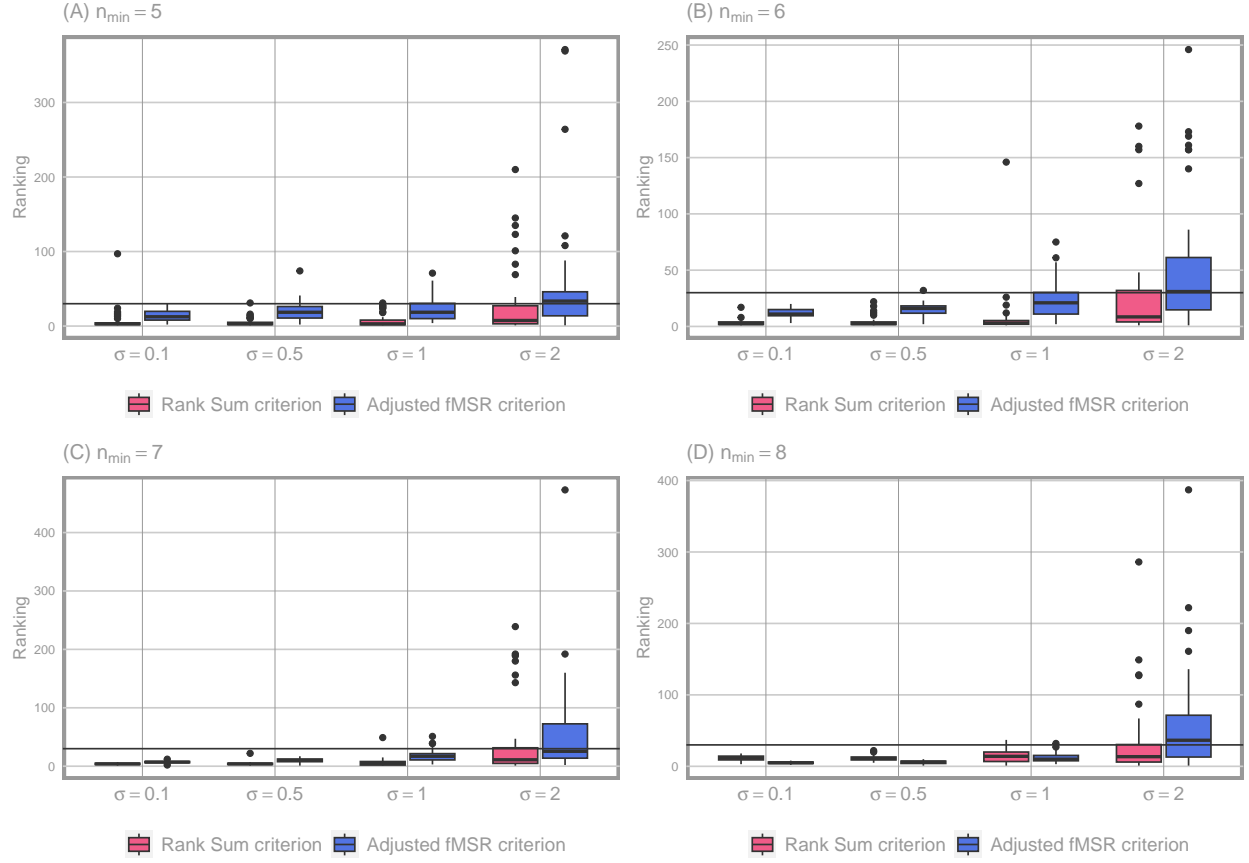

Figure S8: Ranking of the results of *funBAlign* which are most similar to the intentionally embedded motifs, for all simulations where motifs have 10 occurrences and shared noise level. The four panels show the ranking of the algorithm run with minimum cardinalities  $n_{\min} = 5, 6, 7, 8$ , respectively, but pooling across 10 alternative motif sets. For each  $\sigma$ , the red and blue boxplots (left and right) represent ranking according to the rank sum and the adjusted fMSR criterion, respectively. horizontal line indicates rank 30.

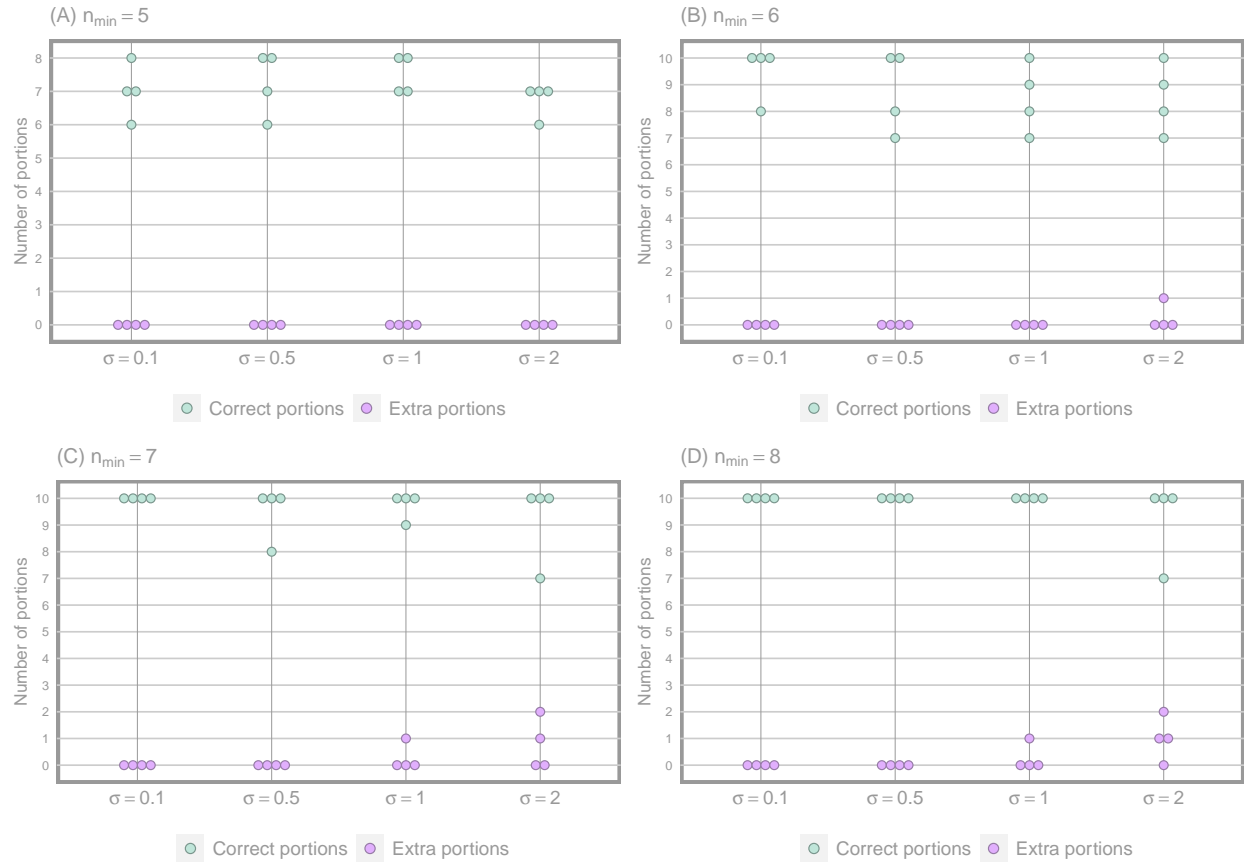

Figure S9: Performance of *funBAlign* for simulations employing motif set n. 7 (where motifs have 10 occurrences and shared noise level), shown separately for runs with varying  $n_{min}$ . Green and pink jittered dots represent correctly identified portions and extra portions, respectively.

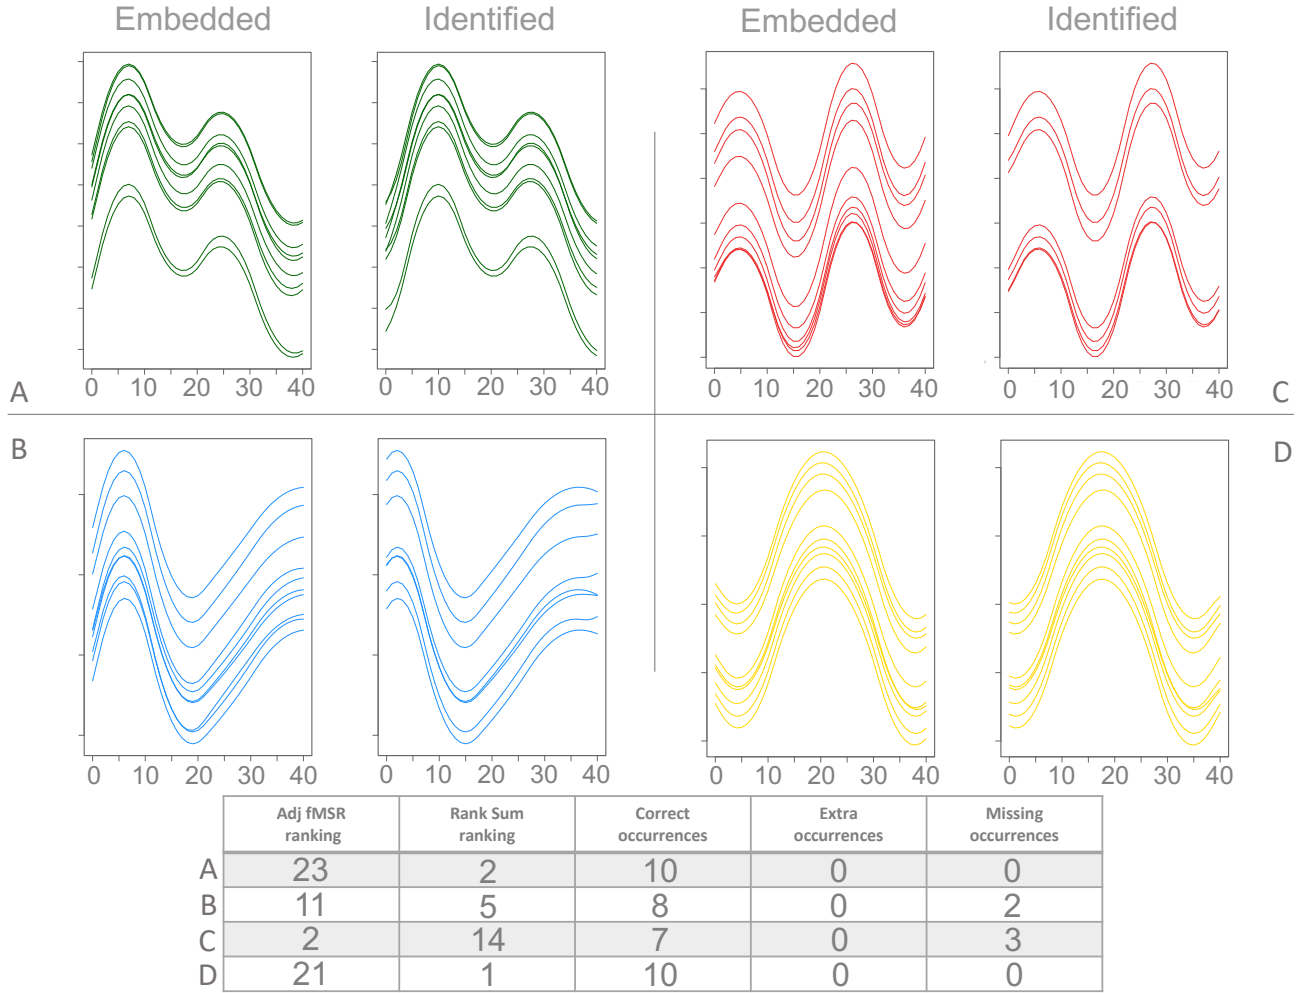

Figure S10: Motif identification for the simulation employing motif set n. 7 and  $\sigma = 0.5$ , where motifs have 10 occurrences. *funB1align* is run with  $n_{min} = 6$ . For each of the 4 motifs, color-coded in green, red, blue and yellow, left and right panels show the 10 occurrences embedded in the curve and the most similar portions identified by the algorithm, respectively. The table provides rankings and numbers of correctly identified, extra and missing occurrences for each motif. No extra occurrences are identified, but 5 embedded occurrences are missed.

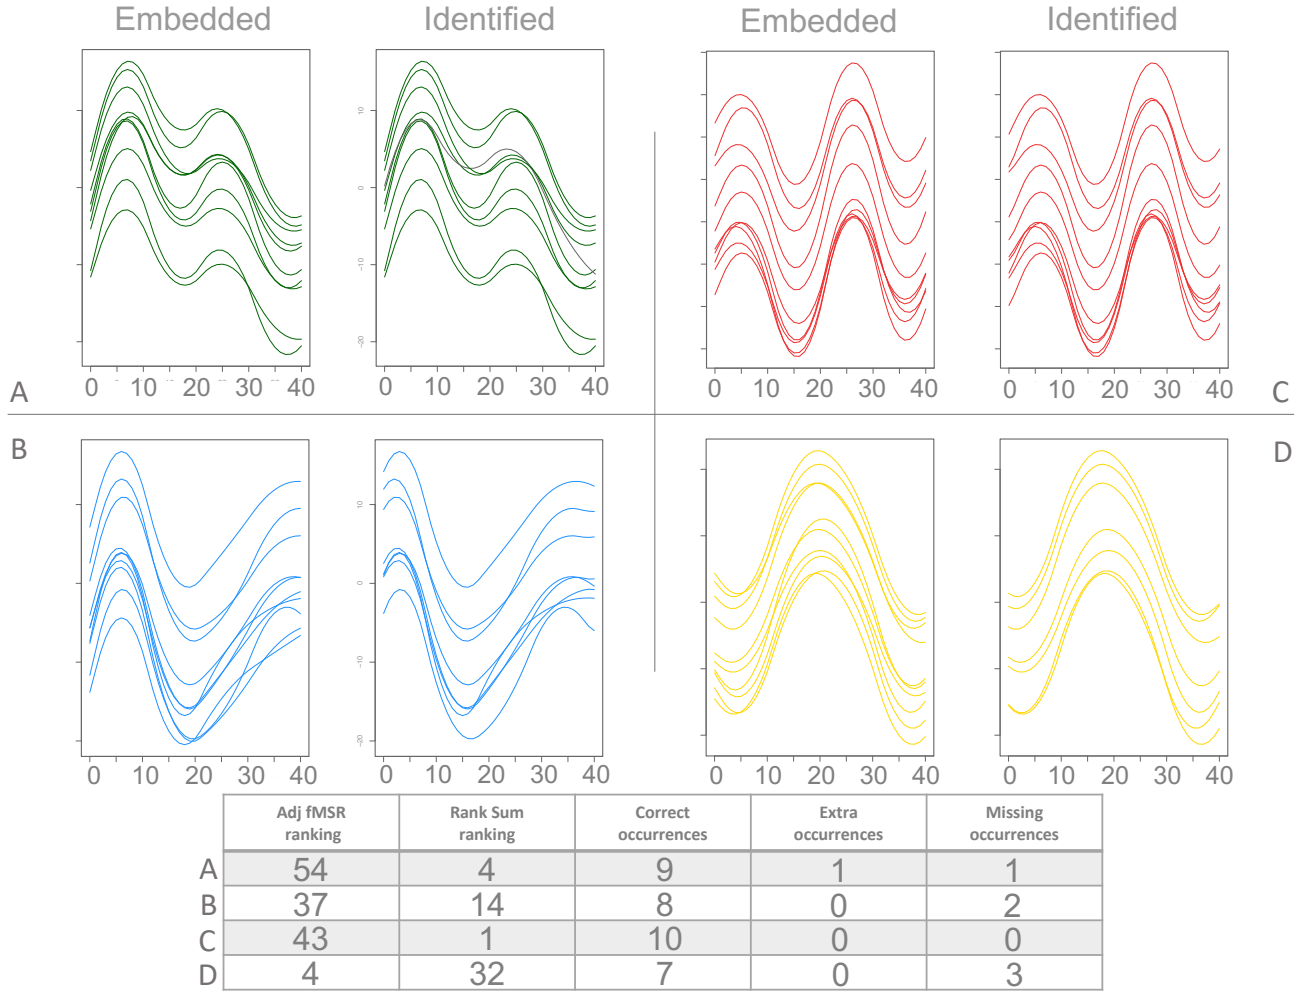

Figure S11: Motif identification for the simulation employing motif set n. 7 and  $\sigma = 2$ , where motifs have 10 occurrences. *funBAlign* is run with  $n_{min} = 6$ . See legend for Figure S10. Extra occurrences are represented in gray among the identified portions panels.

## S4 Motifs with different noise levels

### S4.1 Motifs with 8 occurrences

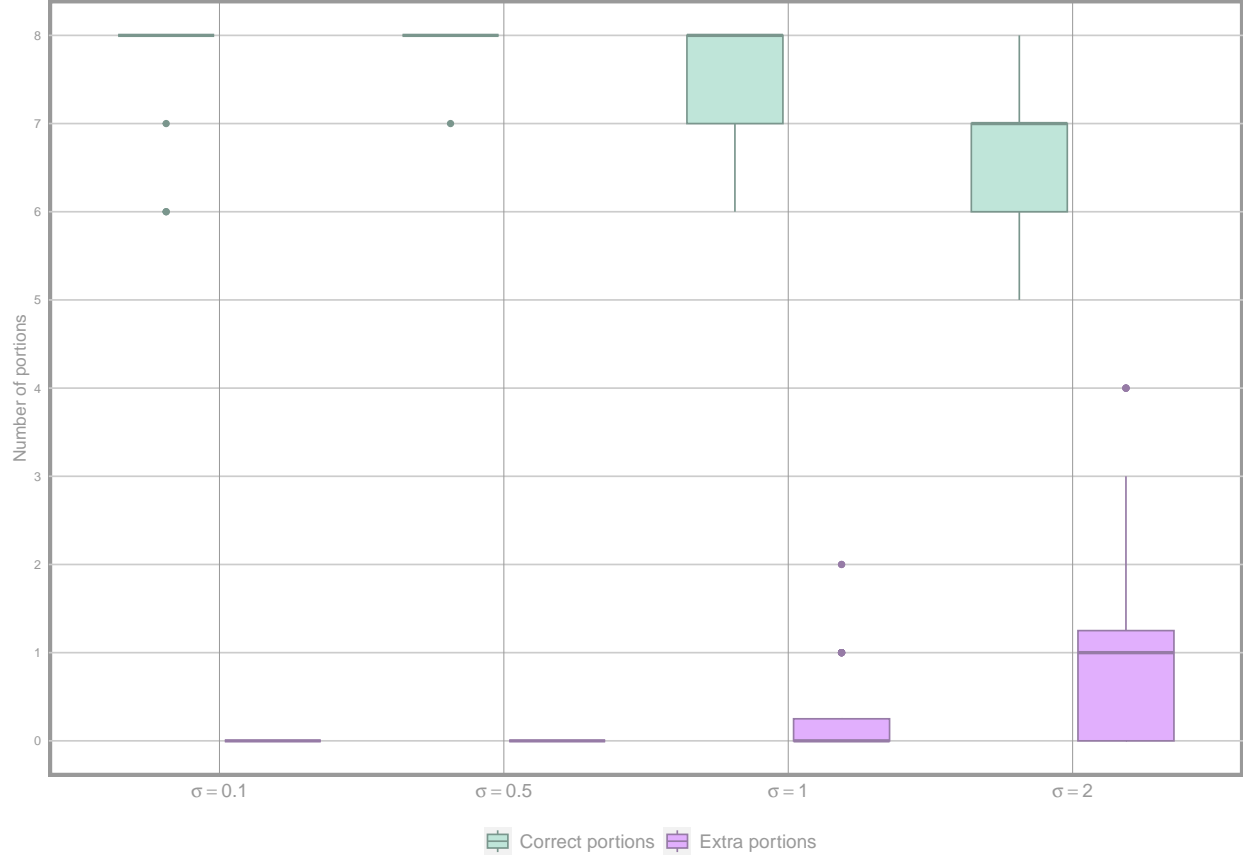

Figure S12: Performance of *funBAlign* for all simulations where motifs have 8 occurrences and different noise levels. The algorithm is run with minimum cardinalities  $n_{min} = 5, 6, 7, 8$  and results are pooled. For each  $\sigma$ , the green and pink boxplots (left and right) represent correctly identified portions and extra portions, respectively. See Figure 2.A.

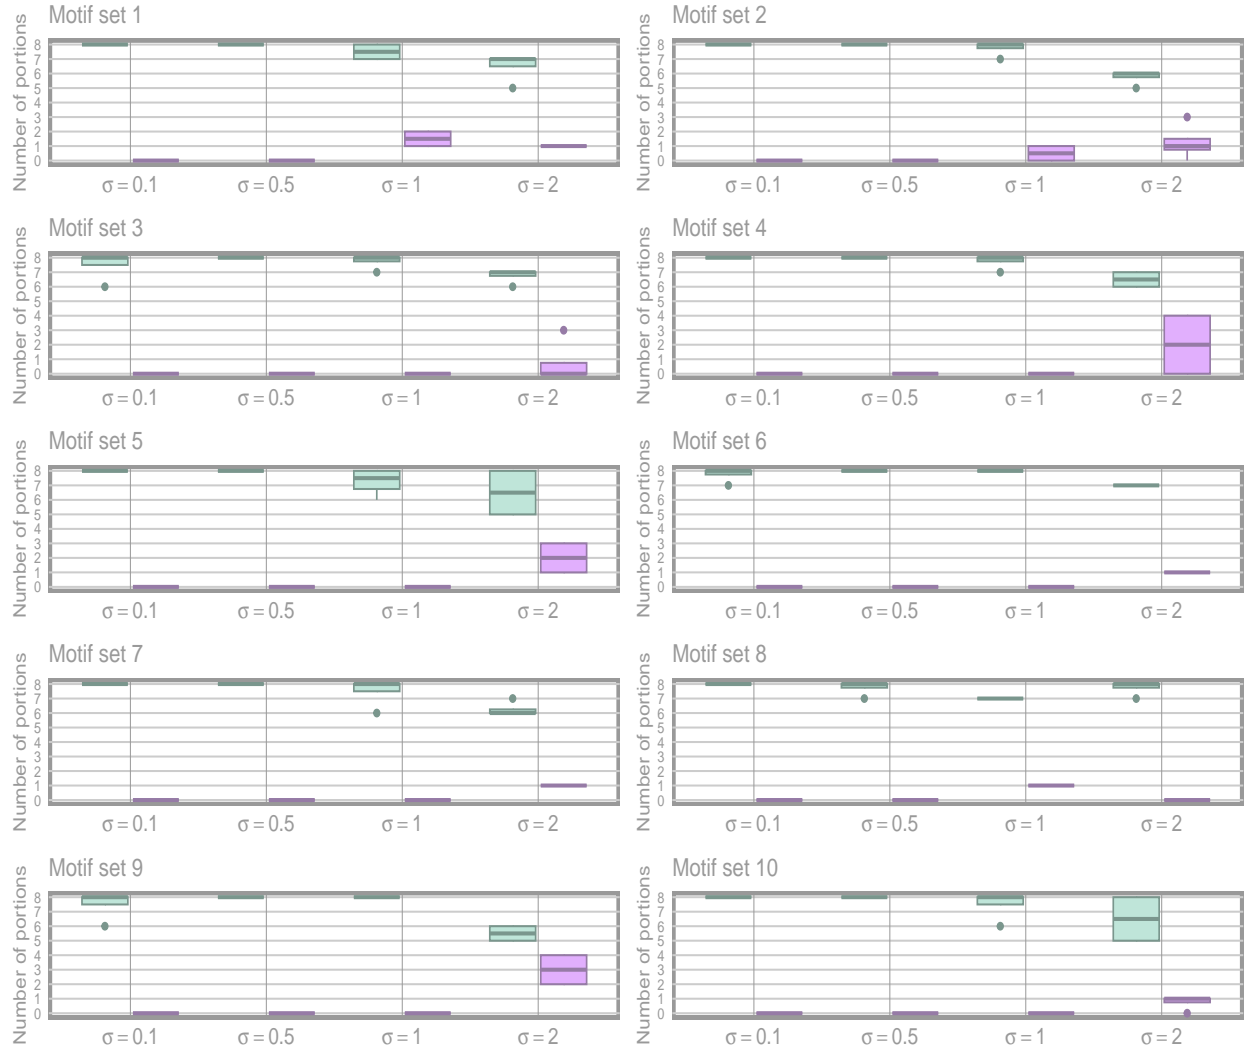

Figure S13: Performance of *funBAlign* for all simulations where motifs have 8 occurrences and different noise level. Different panels show the performance pooling across runs of the algorithm with minimum cardinalities  $n_{min} = 5, 6, 7, 8$ , but separately for each of the 10 alternative motif sets. For each  $\sigma$ , the green and pink boxplots (left and right) represent correctly identified portions and extra portions, respectively.

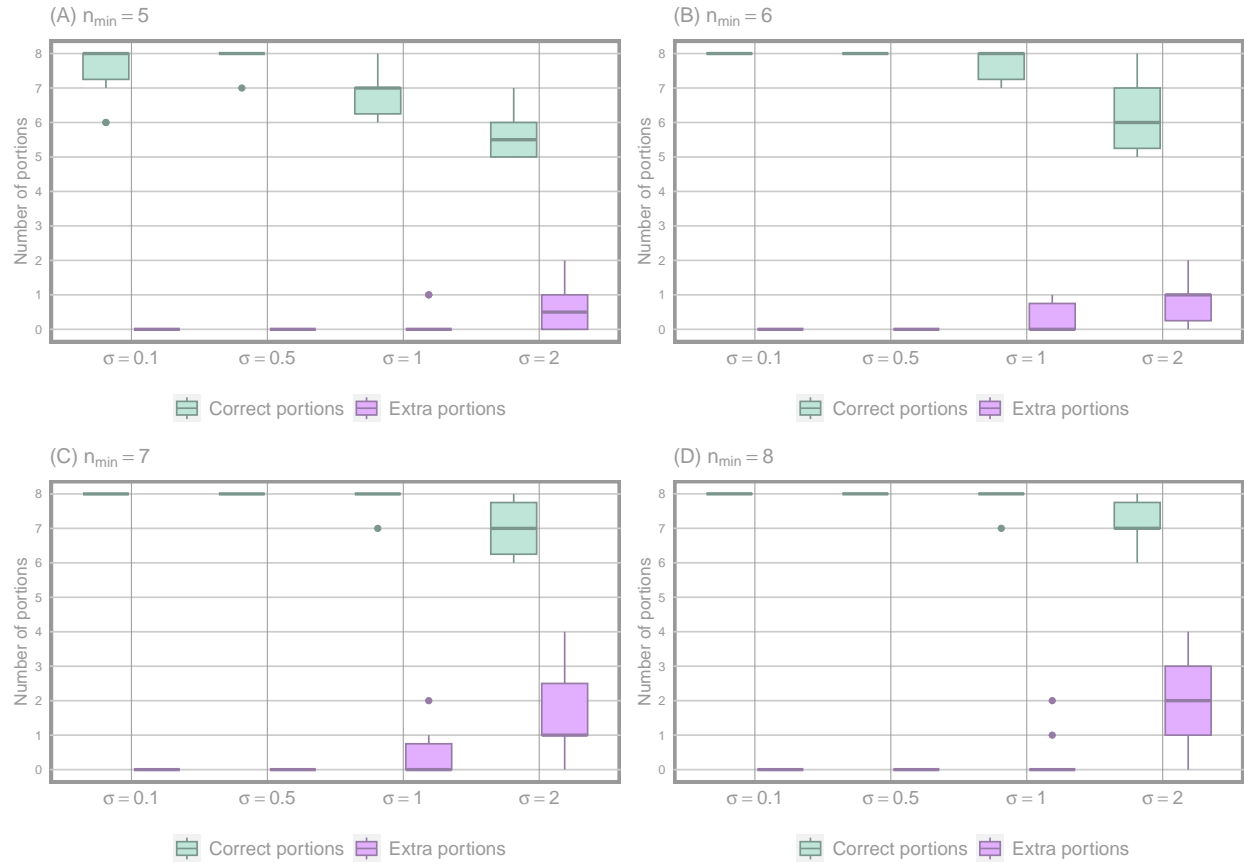

Figure S14: Performance of *funBIalign* for all simulations where motifs have 8 occurrences and different noise level. The four panels show the performance of the algorithm run with minimum cardinalities  $n_{\min} = 5, 6, 7, 8$ , respectively, but pooling across 10 alternative motif sets. For each  $\sigma$ , the green and pink boxplots (left and right) represent correctly identified portions and extra portions, respectively.

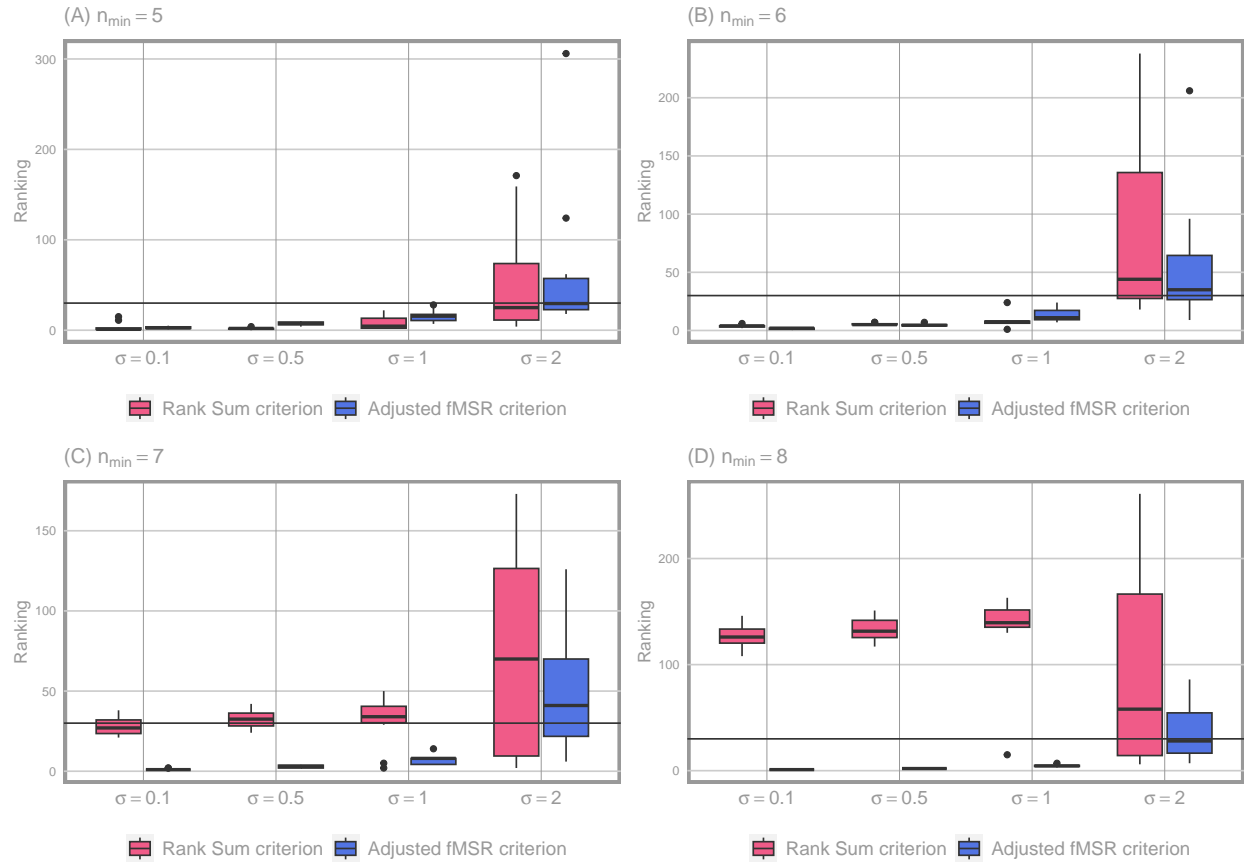

Figure S15: Ranking of the results of *funB1align* which are most similar to the intentionally embedded motifs, for all simulations where motifs have 8 occurrences and different noise level. The four panels show the ranking of the algorithm run with minimum cardinalities  $n_{\min} = 5, 6, 7, 8$ , respectively, but pooling across 10 alternative motif sets. For each  $\sigma$ , the red and blue boxplots (left and right) represent ranking according to the rank sum and the adjusted fMSR criterion, respectively. Horizontal line indicates rank 30.

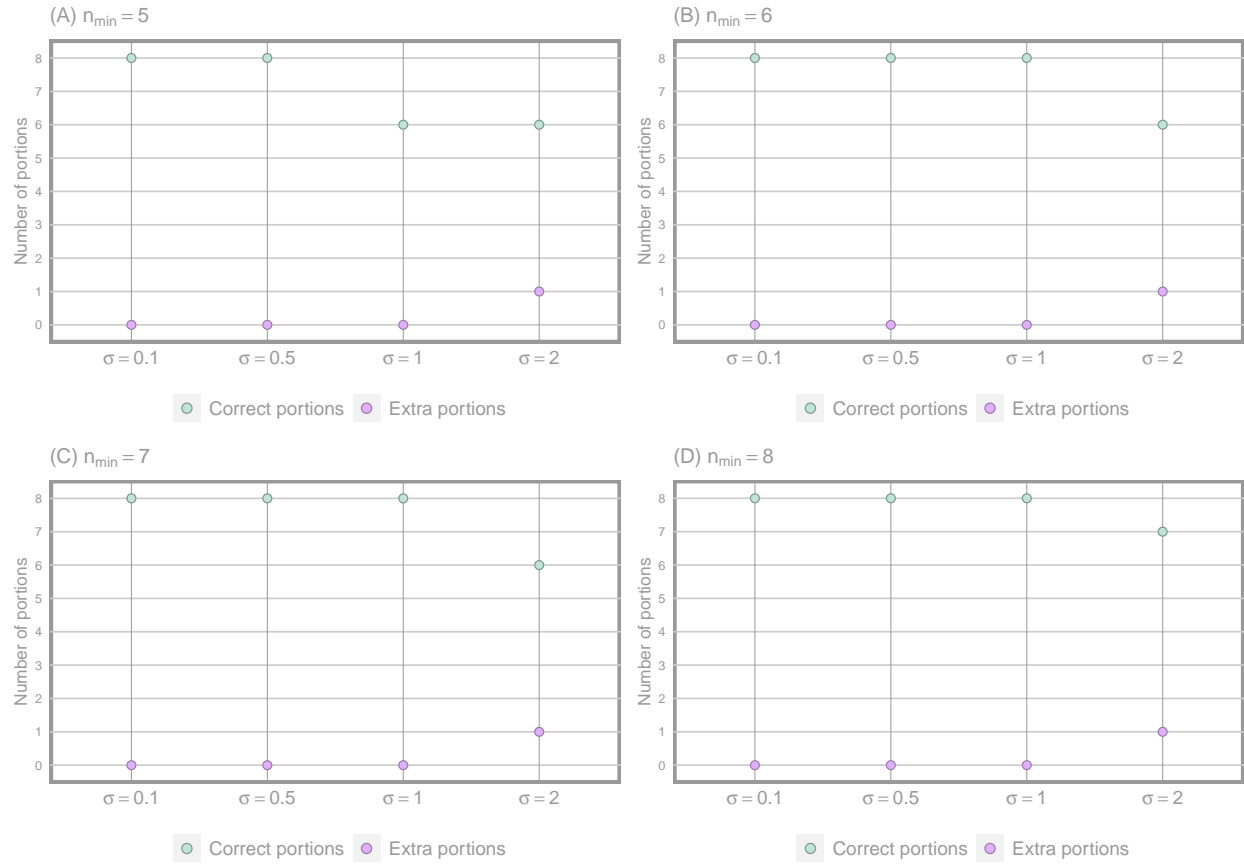

Figure S16: Performance of *funBAlign* for simulations employing motif set n. 7 (where motifs have 8 occurrences and different noise level), shown separately for runs with varying  $n_{\min}$ . Green and pink jittered dots represent correctly identified portions and extra portions, respectively.

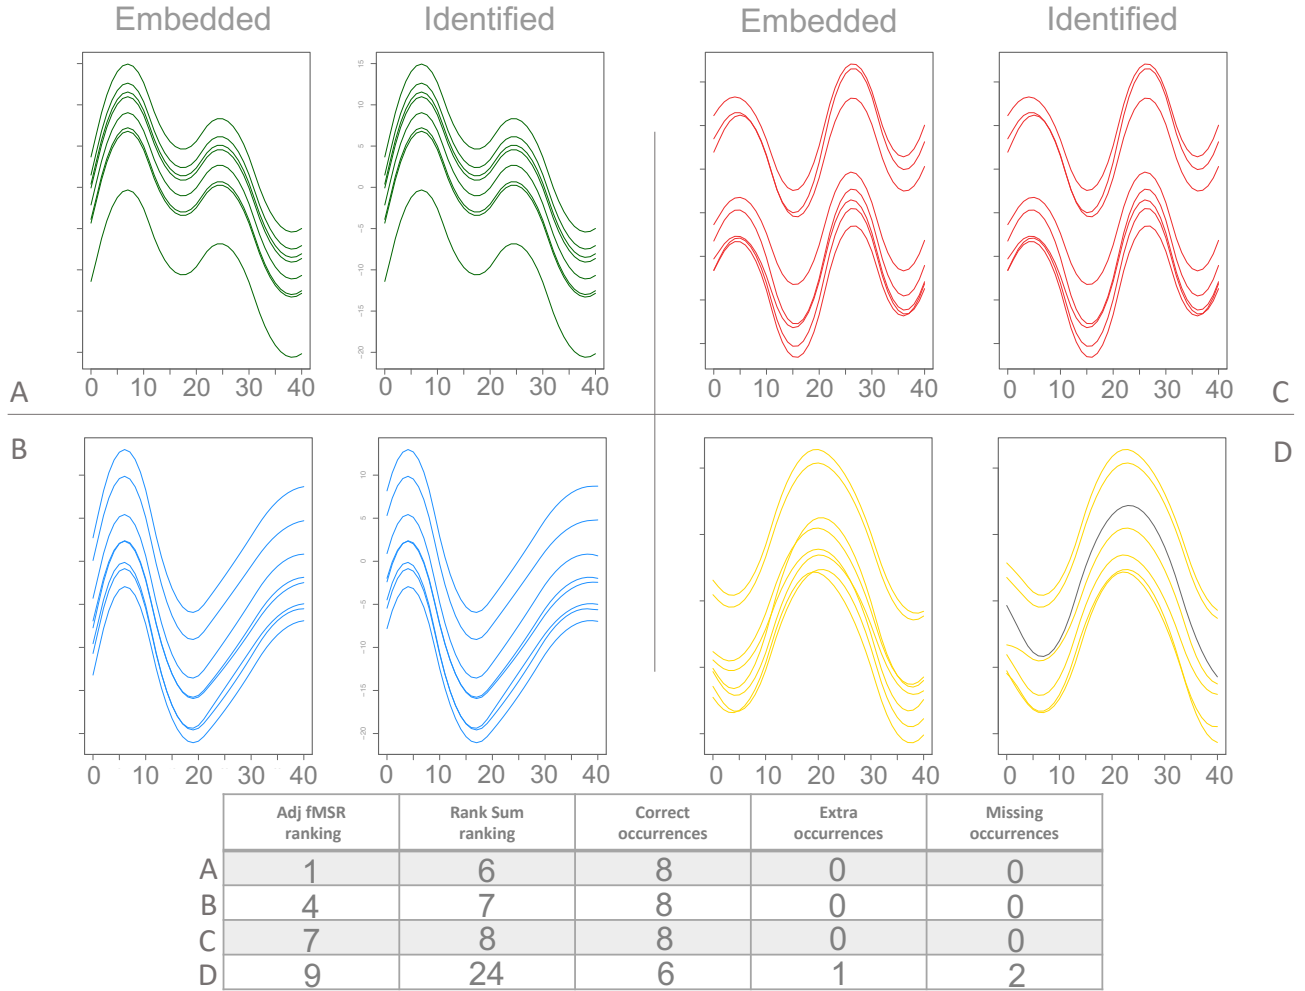

Figure S17: Comparisons between the four embedded motifs (left) and the most similar ones identified by *funBAlign* (right) for motif set n. 7 and different noise level (where motifs have 8 occurrences). The algorithm is run with minimum cardinality  $n_{min} = 6$ . The table reports the ranking according to the adjusted fMSR and the rank sum criteria, as well as details on the number of correct, extra, and missing occurrences.

## S4.2 Motifs with 10 occurrences

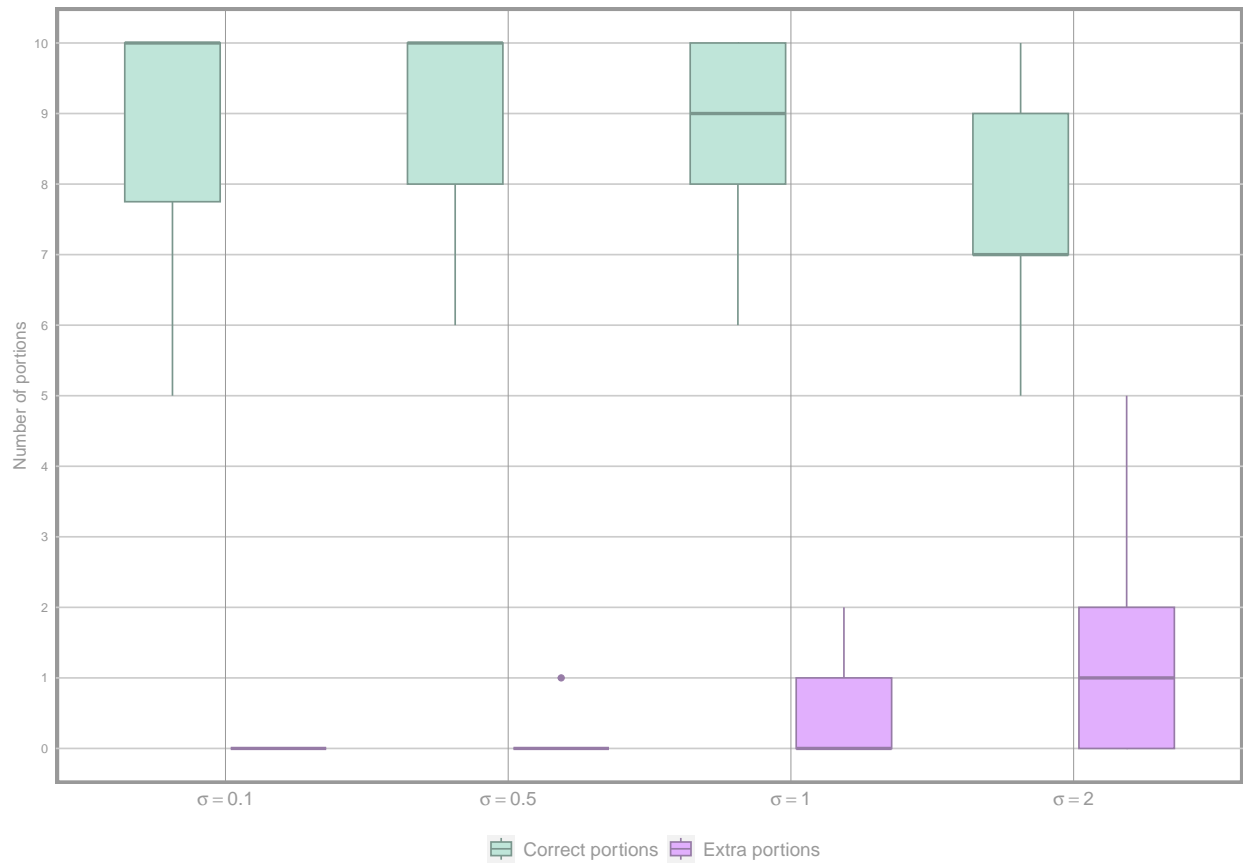

Figure S18: Performance of *funBIalign* for all simulations where motifs have 10 occurrences and different noise levels. The algorithm is run with minimum cardinalities  $n_{min} = 5, 6, 7, 8$  and results are pooled. For each  $\sigma$ , the green and pink boxplots (left and right) represent correctly identified portions and extra portions, respectively. See Figure 2.A.

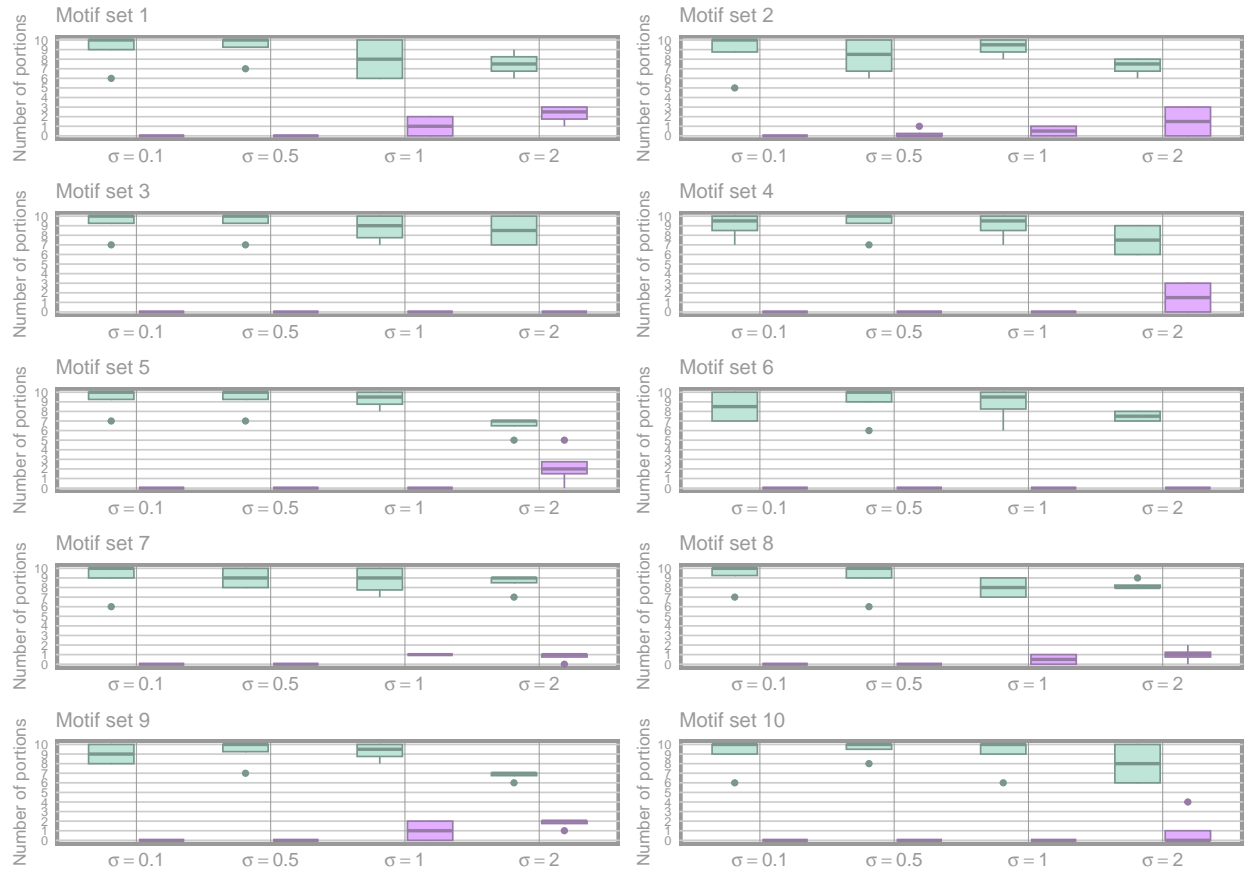

Figure S19: Performance of *funBAlign* for all simulations where motifs have 10 occurrences and different noise level. Different panels show the performance pooling across runs of the algorithm with minimum cardinalities  $n_{min} = 5, 6, 7, 8$ , but separately for each of the 10 alternative motif sets. For each  $\sigma$ , the green and pink boxplots (left and right) represent correctly identified portions and extra portions, respectively.

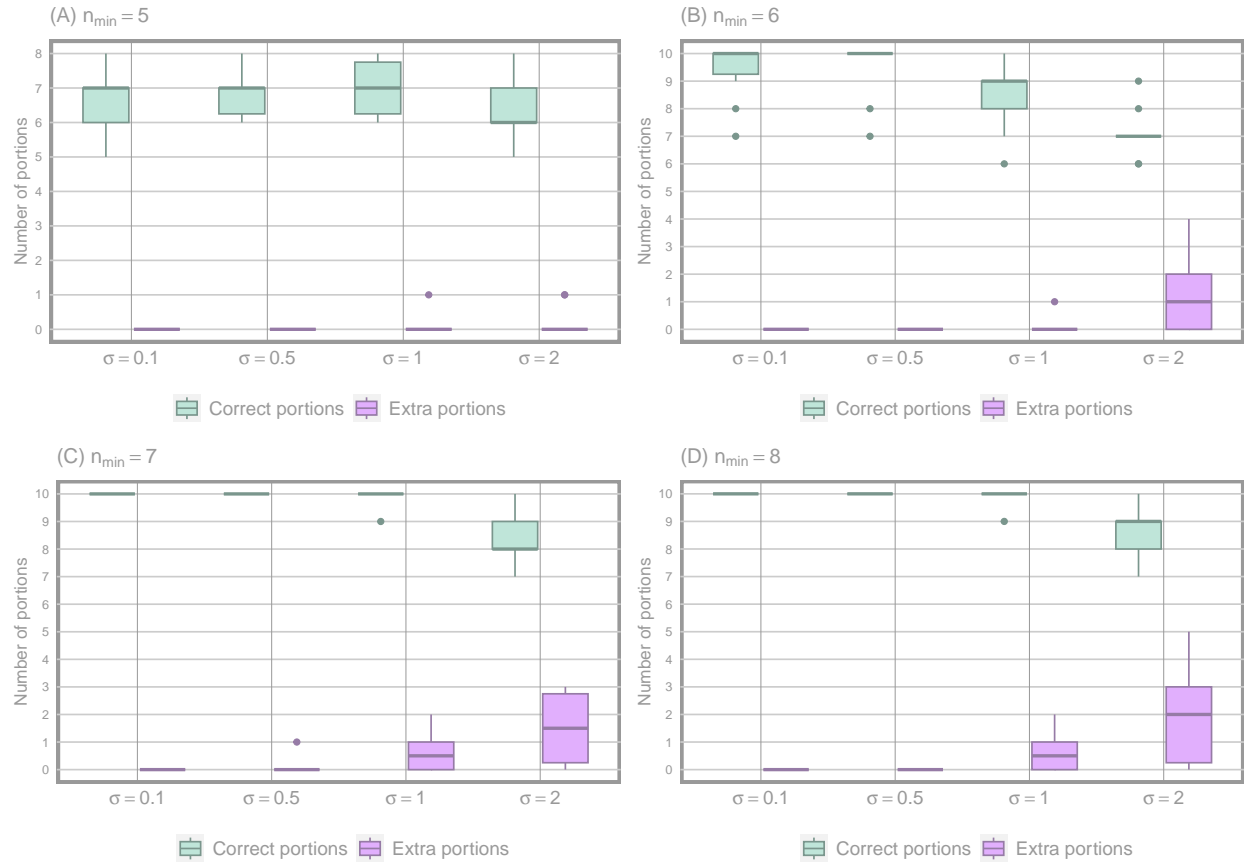

Figure S20: Performance of *funBAlign* for all simulations where motifs have 10 occurrences and different noise level. The four panels show the performance of the algorithm run with minimum cardinalities  $n_{\min} = 5, 6, 7, 8$ , respectively, but pooling across 10 alternative motif sets. For each  $\sigma$ , the green and pink boxplots (left and right) represent correctly identified portions and extra portions, respectively.

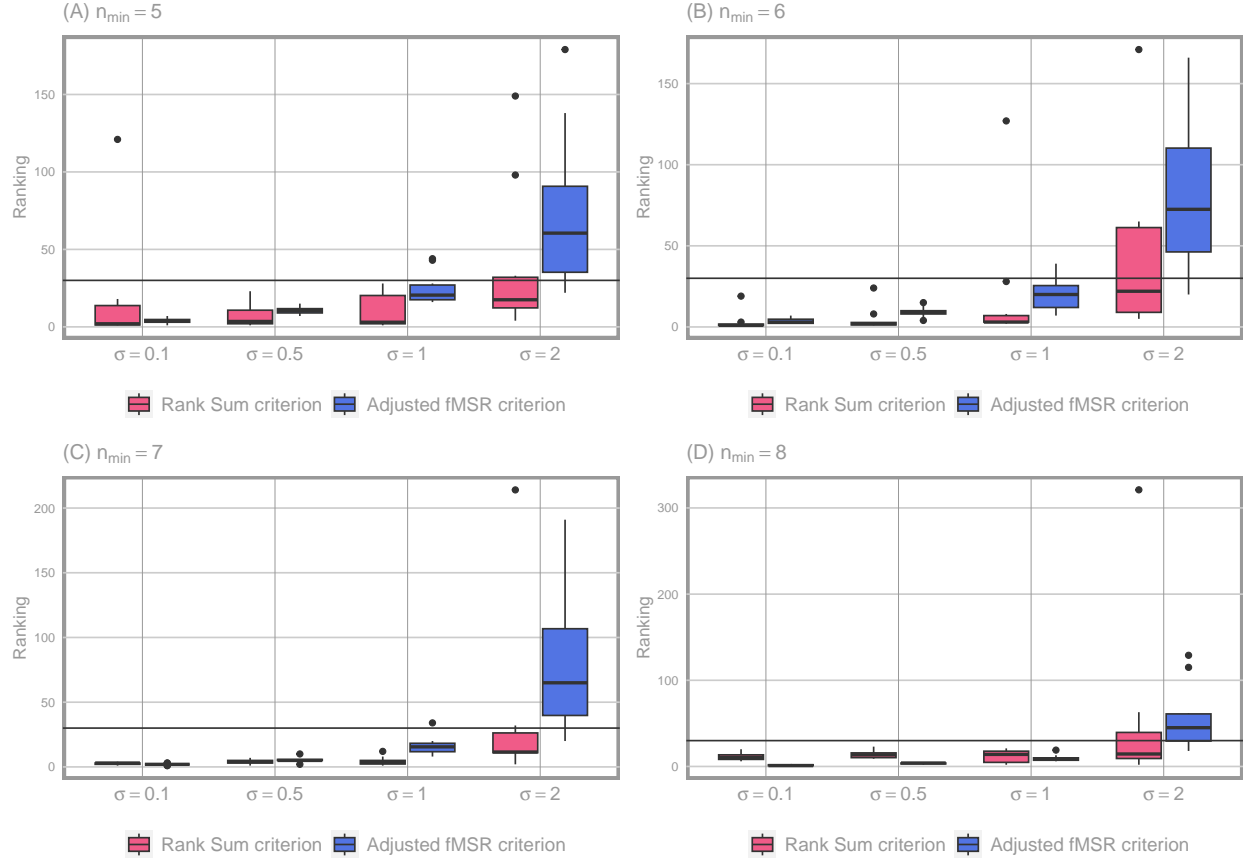

Figure S21: Ranking of the results of *funBAlign* which are most similar to the intentionally embedded motifs, for all simulations where motifs have 10 occurrences and different noise level. The four panels show the ranking of the algorithm run with minimum cardinalities  $n_{\min} = 5, 6, 7, 8$ , respectively, but pooling across 10 alternative motif sets. For each  $\sigma$ , the red and blue boxplots (left and right) represent ranking according to the rank sum and the adjusted fMSR criterion, respectively. Horizontal line indicates rank 30.

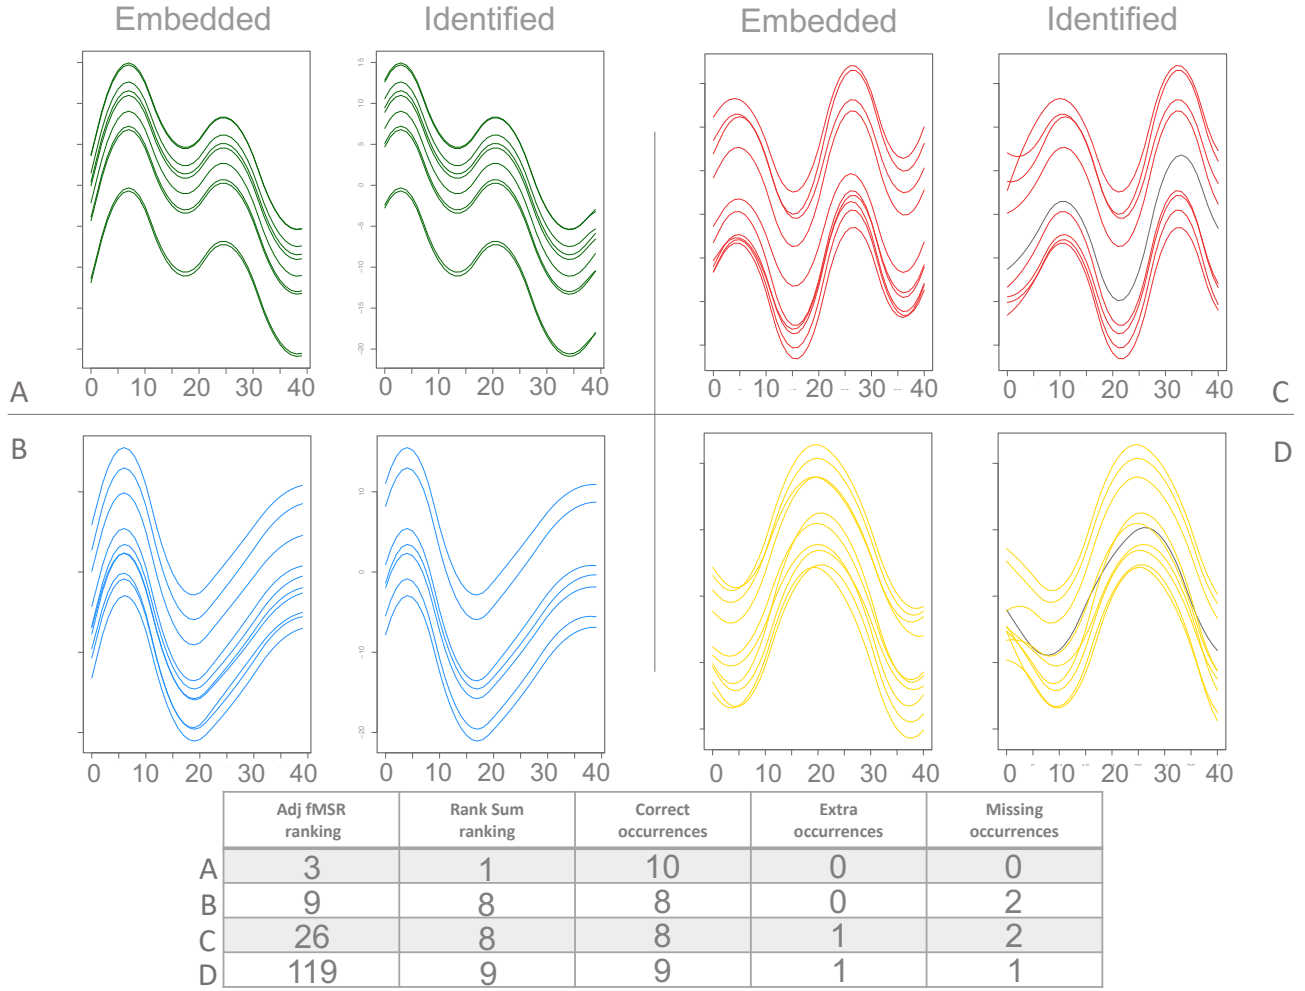

Figure S22: Comparisons between the four embedded motifs (left) and the most similar ones identified by *funBAlign* (right) for motif set n. 7 and different noise level (where motifs have 10 occurrences). The algorithm is run with minimum cardinality  $n_{min} = 6$ . The table reports the ranking according to the adjusted fMSR and the rank sum criteria, as well as details on the number of correct, extra, and missing occurrences.

## S5 Comparison with *SCRIMP-MP*

Table S1 presents the comparison between *funBIalign* and *SCRIMP-MP* in the case of motifs with 8 occurrences each and different noise levels, using motif set n. 7 (see Section 4). As in the comparisons of Section 5, *funBIalign* is run with  $\ell = 41$  (the true length of the motifs) and  $n_{min} = 5, 6, 7, 8$ , while *SCRIMP-MP* is run with  $u = 50$ ,  $\ell = 41$  and all possible combinations of  $R = 3, 10, 25, 50$  and  $k_{neighbor} = 4, 6, 8$ . As expected, the identification of the motifs is harder for the motif with  $\sigma = 2$  with both the methods. In general, *funBIalign* performs better than *SCRIMP-MP*.

| Motif                      | <i>funBIalign</i> - $n_{min}$ |              |              |              | MP             |              | $R$          |              |              |
|----------------------------|-------------------------------|--------------|--------------|--------------|----------------|--------------|--------------|--------------|--------------|
|                            | 5                             | 6            | 7            | 8            | $k_{neighbor}$ | 3            | 10           | 25           | 50           |
| Motif 1 ( $\sigma = 0.1$ ) | <b>(8,0)</b>                  | <b>(8,0)</b> | <b>(8,0)</b> | <b>(8,0)</b> | 4              | (6,0)        | (6,0)        | (6,0)        | (6,0)        |
|                            |                               |              |              |              | 6              | (7,0)        | <b>(8,0)</b> | <b>(8,0)</b> | <b>(8,0)</b> |
|                            |                               |              |              |              | 8              | (7,0)        | <b>(8,0)</b> | <b>(8,0)</b> | <b>(8,0)</b> |
| Motif 2 ( $\sigma = 0.5$ ) | <b>(8,0)</b>                  | <b>(8,0)</b> | <b>(8,0)</b> | <b>(8,0)</b> | 4              | (6,0)        | (6,0)        | (6,0)        | (6,0)        |
|                            |                               |              |              |              | 6              | <b>(8,0)</b> | <b>(8,0)</b> | <b>(8,0)</b> | <b>(8,0)</b> |
|                            |                               |              |              |              | 8              | <b>(8,0)</b> | <b>(8,0)</b> | (8,2)        | (8,2)        |
| Motif 3 ( $\sigma = 1$ )   | (6,0)                         | <b>(8,0)</b> | <b>(8,0)</b> | <b>(8,0)</b> | 4              | (6,0)        | (6,0)        | (6,0)        | (6,0)        |
|                            |                               |              |              |              | 6              | (7,1)        | (7,1)        | (7,1)        | (7,1)        |
|                            |                               |              |              |              | 8              | (8,1)        | (8,2)        | (8,2)        | (8,2)        |
| Motif 4 ( $\sigma = 2$ )   | (6,1)                         | (6,1)        | (6,1)        | (7,1)        | 4              | (4,2)        | (4,2)        | (4,2)        | (4,2)        |
|                            |                               |              |              |              | 6              | (5,3)        | (5,3)        | (5,3)        | (5,3)        |
|                            |                               |              |              |              | 8              | (6,4)        | (7,3)        | (7,3)        | (7,3)        |

Table S1: Comparison between *funBIalign* and *SCRIMP-MP*. Cases in which all occurrences are correctly identified without the addition of any extra portions are in bold.

## S6 Case studies

### S6.1 Case study 1: Food price inflation

The 19 curves considered in this case study represent the food price inflation measurements for the following geographical regions:

- Eastern Africa
- Middle Africa
- Northern Africa
- Southern Africa
- Western Africa
- Northern America

- Central America
- Caribbean
- South America
- Central Asia
- Eastern Asia
- Southern Asia
- South-eastern Asia
- Western Asia
- Eastern Europe
- Northern Europe
- Southern Europe
- Western Europe
- Oceania

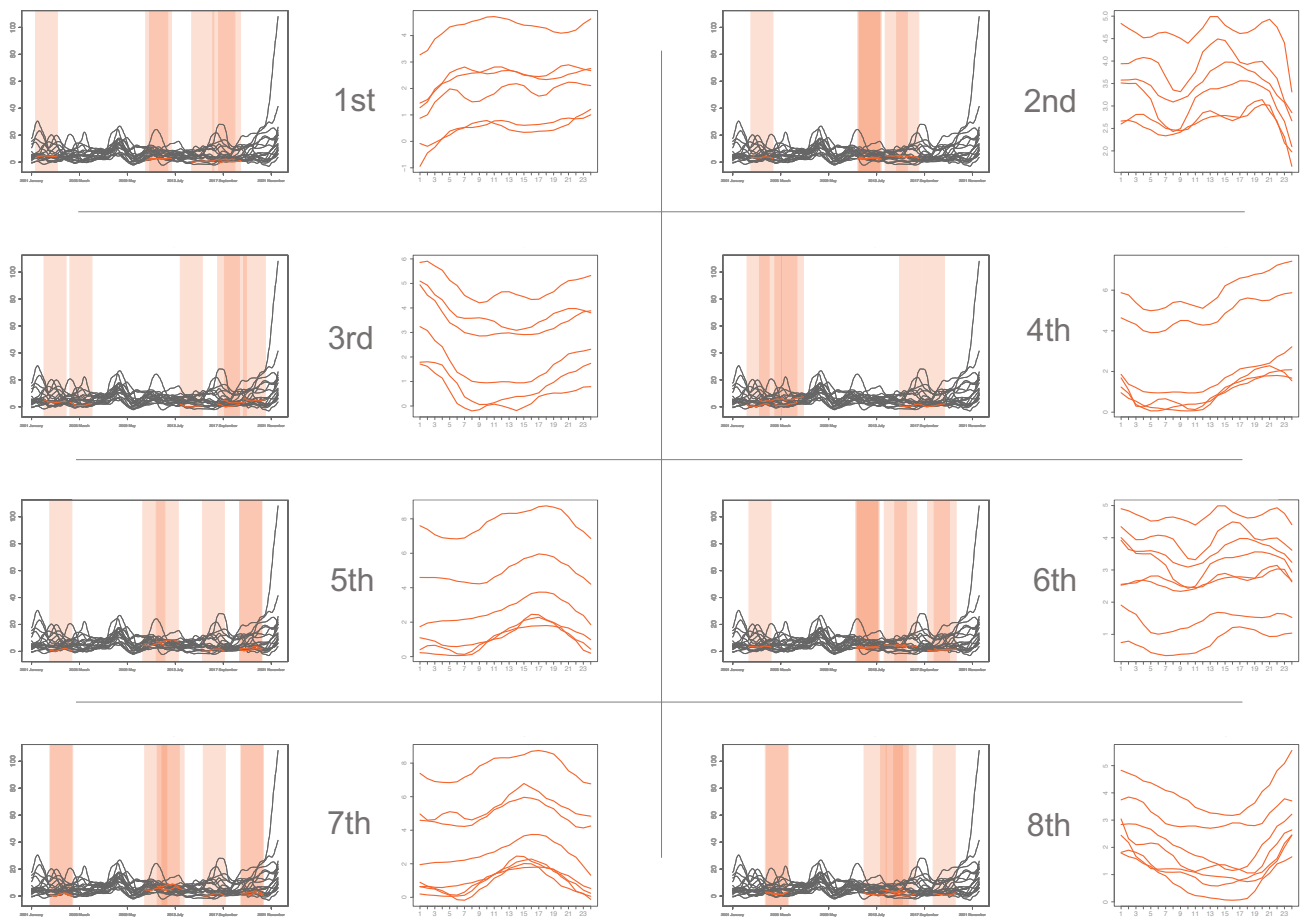

Figure S23: Best 8 motifs according to the adjusted fMSR criterion in the curves for the 19 geographical regions. It is possible to notice how some motif presents occurrences with shared or overlapping domains.

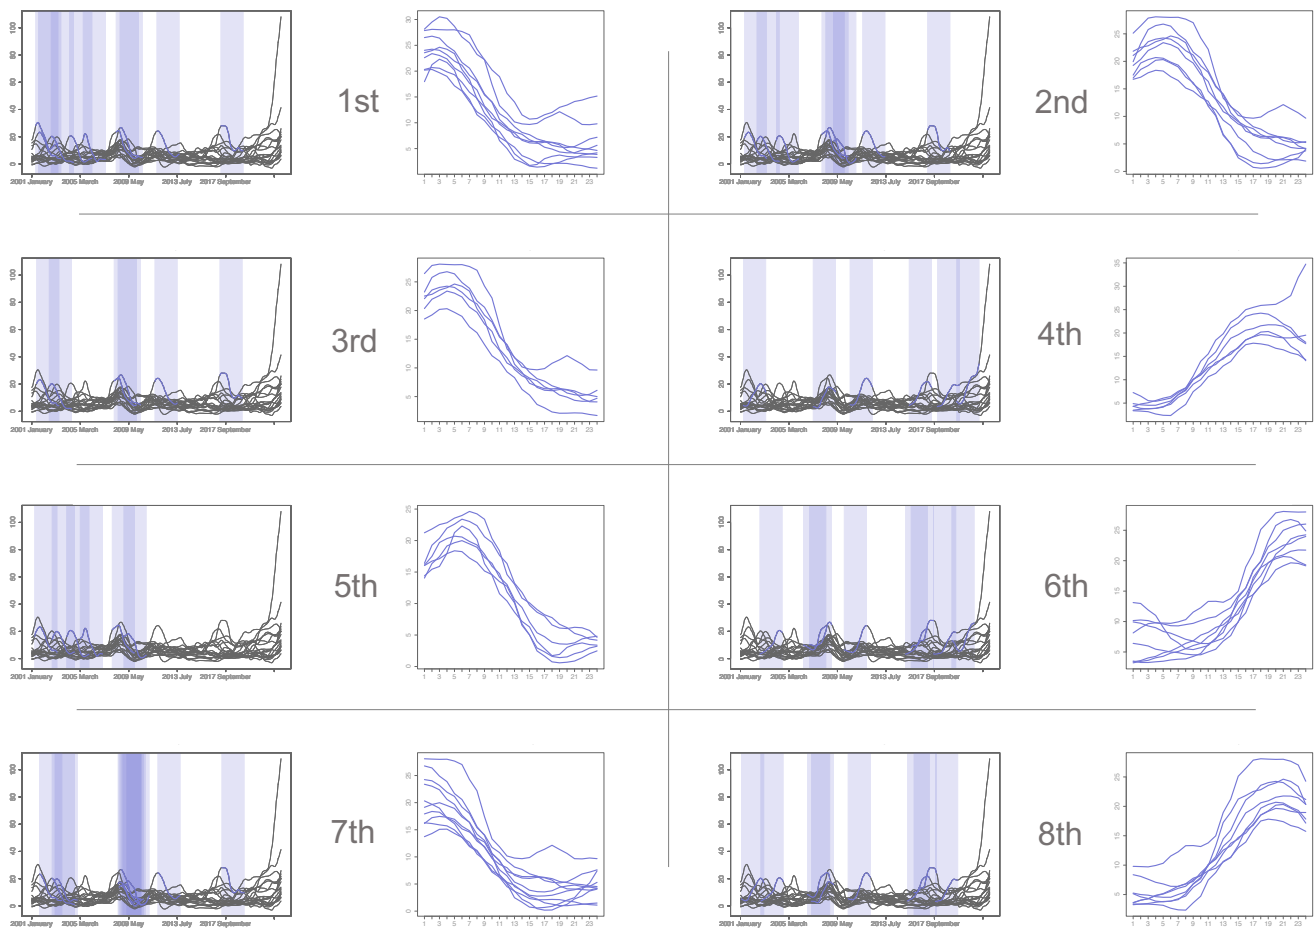

Figure S24: Best 8 motifs according to the variance criterion for the curves for the 19 geographical regions. It is possible to notice how some motif presents occurrences with shared or overlapping domains.

## S6.2 Case study 2: Temperature changes

The 19 curves used in this case study represent the temperature change with respect to a baseline climatology for the following regions:

- Eastern Africa
- Middle Africa
- Northern Africa
- Southern Africa
- Western Africa
- Northern America
- Central America
- Caribbean
- South America
- Central Asia
- Eastern Asia
- Southern Asia
- South-eastern Asia
- Western Asia
- Eastern Europe
- Northern Europe
- Southern Europe
- Western Europe
- Oceania
